# Supplementary material for: Convex Formulation of Overparameterized Deep Neural Networks
Source: arXiv:1911.07626 source file (2019-11-18)
Supplement: Supplementary file 1 [file appendixBackup.tex]

\section{Consistency of Discretization}
\label{apx:discrete-consistency}
In this section, we give the detailed proof of Theorem \ref{theorem:convergence-discrete-NN}, which is comprised of 4 steps. 

\textbf{Step 1.} We first denote $\cZ{L+1}$ to be the set comprised of all the real-valued functions on $\cZ{L}$ and thus we can extend to definitions of $g^{(\ell)}$ in Eqn.\eqref{eq:nn-layer} and $f^{(\ell)}(\rho, z^{(\ell)};x)$ in Eqn.\eqref{eq:nn-activation} to the the case when $\ell=L+1$. Moreover, we need the following definitions:
\begin{align}
    &(1)~\bar{f}^{(\ell)}(z^{(\ell)};x) := h^{(\ell)}\Big(\frac{1}{m^{(\ell-1)}}\sum_{j=1}^{m^{(\ell-1)}} w(z^{(\ell)},z^{(\ell-1)}_j) \hat{f}^{(\ell-1)}_j(x)\Big), \quad \ell=1,\ldots, L+1;\nonumber\\
    &(2)~\bar{g}^{(\ell)}(z^{(\ell)};x):=\frac{1}{m^{(\ell-1)}}\sum_{j=1}^{m^{(\ell-1)}} w(z^{(\ell)},z^{(\ell-1)}_j) \hat{f}^{(\ell-1)}_j(x), \quad \ell=1,\ldots, L+1;\nonumber\\ 
    &(3)~\Delta_1^{(\ell)}\big(z^{(\ell)},z^{(\ell-1)}\big) := \left\| w(z^{(\ell)}, z^{(\ell-1)}) \Big(\bar{f}^{(\ell-1)}(z^{(\ell-1)};x)- f^{(\ell-1)}(\rho, z^{(\ell-1)};x)\Big)\right\|, \quad \ell=2,\ldots, L;\nonumber\\
    &(4)~\Delta_2^{(\ell)}\big(z^{\ell}\big):=\left\|\frac{1}{m^{(\ell-1)}} \sum_{j=1}^{m^{(\ell-1)}} w(z^{(\ell)}, z^{(\ell-1)}_j) f^{(\ell-1)}(\rho, z^{(\ell-1)}_j;x)-g^{(\ell)}(\rho, z^{(\ell)};x)\right\|, \quad \ell=2,\ldots,L;\nonumber\\
    &(5)~A(k,\ell) = \begin{cases}
        1 \mbox{ if }k=0; \\
        \left|\Pi_{j=\ell-k+1}^{\ell}w(z^{(j)},z^{(j-1)})\right|, \mbox{ else if }  0<k\leq \ell;
    \end{cases} ~~ \ell = 1,\ldots, L+1.\nonumber
\end{align}
We notice that actually $\bar{f}^{(\ell)}, \bar{g}^{(\ell)}$ and $\Delta_2^{(\ell)}$ depend on both $z^{(\ell)}$ and $z^{(\ell-1)}_j$ with $j\in [m^{(\ell-1)}]$, for the sake of simplicity, we omit $z^{(\ell-1)}_j$ in the definitions. 


Obviously, it holds that $\bar{f}^{(\ell)}(z^{(\ell)}_j;x)=h^{(\ell)}\big(\bar{g}^{(\ell)}(z^{(\ell)}_j;x)\big)=\hat{f}^{(\ell)}_j(x)$ for all $j\in [m^{(\ell)}]$ and $\ell\in \{1,\ldots, L\}$. 

\textbf{Step 2.} Before giving the formal proof, we present the following lemma, which is needed when we  prove Theorem \ref{theorem:convergence-discrete-NN}. 
\begin{lemma}\label{lemma:Delta-1-2}
	Given a function $B(z^{(\ell)},\ldots, z^{(L)})$ satisfying that $B(z^{(\ell)},\ldots, z^{(L)})\geq 0$ holds for all $z^{(k)}\in \cZ{k}$ with $k=\ell,\ldots, L$ and all $\ell\geq 2$, then we have 
\begin{align} 
\E_{z^{(1)},\ldots,z^{(L)}}B(z^{(\ell)},\ldots, z^{(L)})\Delta_1^{(\ell)}\big(z^{(\ell)},z^{(\ell-1)}\big)\leq& \E_{z^{(1)},\ldots,z^{(L)}}\tilde{B}(z^{(\ell-1)},\ldots, z^{(L)})\Delta_1^{(\ell-1)}(z^{(\ell-1)},z^{(\ell-2)})\nonumber\\
&+\E_{z^{(\ell-2)},\ldots,z^{(L)}}\tilde{B}(z^{(\ell-1)},\ldots, z^{(L)})\Delta_2^{(\ell-1)}(z^{(\ell-1)}),\nonumber
\end{align}	
where $\tilde{B}(z^{(\ell-1)},\ldots, z^{(L)}) = B(z^{(\ell)},\ldots, z^{(L)})\left|w(z^{(\ell)}, z^{(\ell-1)})\right|c_0$.
\end{lemma}
\begin{proof} of Lemma \ref{lemma:Delta-1-2}:\\
From the definition of $\Delta_1^{(\ell)}\big(z^{(\ell)},z^{(\ell-1)}\big)$, we have
	\begin{align}
	&B(z^{(\ell)},\ldots, z^{(L)})\Delta_1^{(\ell)}\big(z^{(\ell)},z^{(\ell-1)}\big)\nonumber\\
	=&B(z^{(\ell)},\ldots, z^{(L)})\left\| w(z^{(\ell)}, z^{(\ell-1)}) \Big(\bar{f}^{(\ell-1)}(z^{(\ell-1)};x)- f^{(\ell-1)}(\rho, z^{(\ell-1)};x)\Big)\right\|\nonumber\\
	=&B(z^{(\ell)},\ldots, z^{(L)})\left|w(z^{(\ell)}, z^{(\ell-1)})\right| \left\| h^{(\ell-1)}\big(\bar{g}^{(\ell-1)}(z^{(\ell-1)};x)\big)-h^{(\ell-1)}\big(g^{(\ell-1)}(\rho,z^{(\ell-1)};x)\big)\right\|\nonumber\\
	\leq&B(z^{(\ell)},\ldots, z^{(L)})\left|w(z^{(\ell)}, z^{(\ell-1)})\right|c_0\left\| \bar{g}(z^{(\ell-1)};x)-g^{(\ell-1)}(\rho,z^{(\ell-1)};x)\right\|\nonumber\\
	\leq&\tilde{B}(z^{(\ell-1)},\ldots, z^{(L)})\left\| \bar{g}(z^{(\ell-1)};x)-g^{(\ell-1)}(\rho,z^{(\ell-1)};x)\right\|\nonumber\\
	\leq&\tilde{B}(z^{(\ell-1)},\ldots, z^{(L)})\frac{1}{m^{(\ell-2)}}\left\|\sum_{j=1}^{m^{(\ell-2)}} w(z^{(\ell-1)},z^{(\ell-2)}_j)\Big( \bar{f}^{(\ell-2)}(z^{(\ell-2)}_j;x)-f^{(\ell-2)}(\rho, z^{(\ell-2)}_j;x)\Big)\right\|\nonumber\\
	&+\tilde{B}(z^{(\ell-1)},\ldots, z^{(L)})\left\|\frac{1}{m^{(\ell-2)}}\sum_{j=1}^{m^{(\ell-2)}} w(z^{(\ell-1)},z^{(\ell-2)}_j)f^{(\ell-2)}(\rho,z^{(\ell-2)}_j;x)-g^{(\ell-1)}(\rho, z^{(\ell-1)};x)\right\|\nonumber\\
		\leq&\tilde{B}(z^{(\ell-1)},\ldots, z^{(L)})\frac{1}{m^{(\ell-2)}}\sum_{j=1}^{m^{(\ell-2)}}\left\| w(z^{(\ell-1)},z^{(\ell-2)}_j)\Big( \bar{f}^{(\ell-2)}(z^{(\ell-2)}_j;x)-f^{(\ell-2)}(\rho, z^{(\ell-2)}_j;x)\Big)\right\|\nonumber\\
	&+\tilde{B}(z^{(\ell-1)},\ldots, z^{(L)})\left\|\frac{1}{m^{(\ell-2)}}\sum_{j=1}^{m^{(\ell-2)}} w(z^{(\ell-1)},z^{(\ell-2)}_j)f^{(\ell-2)}(\rho,z^{(\ell-2)}_j;x)-g^{(\ell-1)}(\rho, z^{(\ell-1)};x)\right\|\nonumber\\
	=& \tilde{B}(z^{(\ell-1)},\ldots, z^{(L)})\Big(\frac{1}{m^{(\ell-2)}}\sum_{j=1}^{m^{(\ell-2)}}\Delta_1^{(\ell-1)}\big(z^{(\ell-1)}, z^{(\ell-2)}_j\big) + \Delta_2^{(\ell-1)}\big(z^{(\ell-1)}\big)\Big).\nonumber
	\end{align}
	Therefore, we have
	\begin{align}
	&\E_{z^{(1)},\ldots,z^{(L)}}B(z^{(\ell)},\ldots, z^{(L)})\Delta_1^{(\ell)}\big(z^{(\ell)},z^{(\ell-1)}\big)\nonumber\\
	\leq&\E_{z^{(1)},\ldots,z^{(L)}}\tilde{B}(z^{(\ell-1)},\ldots, z^{(L)})\Big(\frac{1}{m^{(\ell-2)}}\sum_{j=1}^{m^{(\ell-2)}}\Delta_1^{(\ell-1)}\big(z^{(\ell-1)}, z^{(\ell-2)}_j\big) + \Delta_2^{(\ell-1)}\big(z^{(\ell-1)}\big)\Big)\nonumber\\
	=&\E_{z^{(1)},\ldots,z^{(L)}}\tilde{B}(z^{(\ell-1)},\ldots, z^{(L)})\Delta_1^{(\ell-1)}(z^{(\ell-1)},z^{(\ell-2)})+\E_{z^{(1)},\ldots,z^{(L)}}\tilde{B}(z^{(\ell-1)},\ldots, z^{(L)})\Delta_2^{(\ell-1)}\big(z^{(\ell-1)}\big)\nonumber\\
	=&\E_{z^{(1)},\ldots,z^{(L)}}\tilde{B}(z^{(\ell-1)},\ldots, z^{(L)})\Delta_1^{(\ell-1)}(z^{(\ell-1)},z^{(\ell-2)})+\E_{z^{(\ell-2)},\ldots,z^{(L)}}\tilde{B}(z^{(\ell-1)},\ldots, z^{(L)})\Delta_2^{(\ell-1)}(z^{(\ell-1)})\nonumber
	\end{align}
	The last equality holds since the random variables in $\Delta_2^{(\ell-1)}(z^{(\ell-1)})$ are $z^{(\ell-1)}$ and $z^{(\ell-2)}_j$ with $j\in [m^{(\ell-2)}]$.
	
	The proof is complete.
\end{proof}

\textbf{Step 3.}To avoid avoid redundancy, we first  present the Lemma below. And then in next step we will show that the conclusions (i) and (ii) of Theorem \ref{theorem:convergence-discrete-NN} would either be the special case of or can be derived from this lemma directly.
\begin{lemma}\label{lemma:convergence-discrete-NN}
Suppose that $w^{(\ell)}_{j,k} = w(z^{(\ell)}_j,z^{(\ell-1)}_k)$ with $z^{(\ell)}_j \sim \rho^{(\ell)}, \ell=\{1, \ldots, L\}$. For  $z^{(\ell+1)}\in \cZ{\ell+1}$, we have
\begin{align}
\lim_{m^{(k)}\rightarrow \infty, k=1,\ldots,\ell}\E_{z^{(1)},\ldots, z^{(\ell)}}\; \left\|\bar{f}^{(\ell+1)}(z^{(\ell+1)};x)-f^{(\ell+1)}(\rho, z^{(\ell+1)};x)\right\|=0,\quad \ell = 1,\ldots,L.\nonumber
\end{align}
\end{lemma}
\begin{proof} of Lemma \ref{lemma:convergence-discrete-NN}:\\
From the definition of $\bar{f}^{(\ell+1)}(z^{(\ell+1)};x)$ and $f^{(\ell+1)}(\rho,z^{(\ell+1)}; x)$, we have 
\begin{align}
&\E_{z^{(1)},\ldots, z^{(\ell)}}\;\left\|\bar{f}^{(\ell+1)}(z^{(\ell+1)};x)- f^{(\ell+1)}(\rho, z^{(\ell+1)}; x)\right\|\nonumber\\
=&  \E_{z^{(1)},\ldots, z^{(\ell)}}\;\left\|h^{(\ell+1)}\big(\bar{g}^{(\ell+1)}(z^{\ell+1};x)\big)-h^{(\ell+1)}\big(g^{(\ell+1)}(\rho, z^{(\ell+1)}; x)\big)\right\|\nonumber\\
\leq&\E_{z^{(1)},\ldots, z^{(\ell)}}\;c_0\left\|\bar{g}^{(\ell+1)}(z^{(\ell+1)};x)-g^{(\ell+1)}(\rho, z^{(\ell+1)}; x) \right\|\label{eqn:diff-hfkj-fkj-bound}
\end{align}
For $\left\|\bar{g}^{(\ell+1)}(z^{(\ell+1)};x)-g^{(\ell+1)}(\rho, z^{(\ell+1)}; x) \right\|$, we have
\begin{align}
&\left\|\bar{g}^{(\ell+1)}(z^{(\ell+1)};x)-g^{(\ell+1)}(\rho,z^{(\ell+1)};x) \right\|\nonumber\\
=&\left\|\frac{1}{m^{(\ell)}} \sum_{j=1}^{m^{(\ell)}} w(z^{(\ell+1)}, z^{\ell)}_j) \hat{f}^{(\ell)}_j(x)-g^{(\ell+1)}(\rho,z^{(\ell+1)};x) \right\|\nonumber\\
\leq& \left\|\frac{1}{m^{(\ell)}} \sum_{j=1}^{m^{(\ell)}} w(z^{(\ell+1)}, z^{(\ell)}_j) \Big(\bar{f}^{(\ell)}(z^{(\ell)}_j;x)- f^{(\ell)}(\rho, z^{(\ell)}_j;x)\Big)\right\|\nonumber\\
&+\left\|\frac{1}{m^{(\ell)}} \sum_{j=1}^{m^{(\ell)}} w(z^{(\ell+1)}, z^{(\ell)}_j) f^{(\ell)}(\rho, z^{(\ell)}_j;x)-g^{(\ell+1)}(\rho,z^{(\ell+1)};x)\right\|\nonumber\\
=& \left\|\frac{1}{m^{(\ell)}} \sum_{j=1}^{m^{(\ell)}} w(z^{(\ell+1)}, z^{(\ell)}_j) \Big(\bar{f}^{(\ell)}(z^{(\ell)}_j;x)- f^{(\ell)}(\rho, z^{(\ell)}_j;x)\Big)\right\| + \Delta_2^{(\ell+1)}\big(z^{(\ell+1)}\big)\nonumber\\
\leq &  \frac{1}{m^{(\ell)}} \sum_{j=1}^{m^{(\ell)}}\left\| w(z^{(\ell+1)}, z^{(\ell)}_j) \Big(\bar{f}^{(\ell)}(z^{(\ell)}_j;x)- f^{(\ell)}(\rho, z^{(\ell)}_j;x)\Big)\right\| + \Delta_2^{(\ell+1)}\big(z^{(\ell+1)}\big)\nonumber\\
=&\frac{1}{m^{(\ell)}} \sum_{j=1}^{m^{(\ell)}}\Delta_1^{(\ell+1)}\big(z^{(\ell+1)},z^{(\ell)}_j\big) +\Delta_2^{(\ell+1)}\big(z^{(\ell+1)}\big). \label{eqn:bgk-gk-bound}
\end{align}
By substituting Eqn. \eqref{eqn:bgk-gk-bound} into  Eqn. \eqref{eqn:diff-hfkj-fkj-bound}, we have
\begin{align}
&\E_{z^{(1)},\ldots, z^{(\ell)}}\;\left\|\bar{f}^{(\ell+1)}(z^{(\ell+1)};x)- f^{(\ell+1)}(\rho, z^{(\ell+1)}; x)\right\|\nonumber\\
\leq & \E_{z^{(1)},\ldots, z^{(\ell)}}\;c_0\frac{1}{m^{(\ell)}} \sum_{j=1}^{m^{(\ell)}}\Delta_1^{(\ell+1)}\big(z^{(\ell+1)},z^{(\ell)}_j\big) +\E_{z^{(1)},\ldots, z^{(\ell)}}\;c_0\Delta_2^{(\ell+1)}\big(z^{(\ell+1)}\big)\nonumber\\
=&\E_{z^{(1)},\ldots, z^{(\ell)}}\;c_0\Delta_1^{(\ell+1)}\big(z^{(\ell+1)},z^{(\ell)}\big) + \E_{z^{(\ell)}}\;c_0\Delta_2^{(\ell+1)}\big(z^{(\ell+1)}\big).\label{eqn:diff-bf-f-bound}
\end{align}
The last equality holds since the variables $z^{(1)}, \ldots, z^{(\ell-1)}$ are missing in the second item of \eqref{eqn:diff-bf-f-bound}. 

We now turn to consider the item $\Delta_1^{(\ell+1)}\big(z^{(\ell+1)},z^{(\ell)}\big)$ in Eqn.\eqref{eqn:diff-bf-f-bound}. We should point out that we cannot apply Lemma \ref{lemma:Delta-1-2} to it now, since  we do not take expectation on $z^{(\ell+1)}$ in Eqn.\eqref{eqn:diff-bf-f-bound}. By its definition, we have
\begin{align}
&\Delta_1^{(\ell+1)}\big(z^{(\ell+1)},z^{(\ell)}\big)\nonumber\\
=&\left\| w(z^{(\ell+1)}, z^{(\ell)}) \Big(\bar{f}^{(\ell)}(z^{(\ell)};x)- f^{(\ell)}(\rho, z^{(\ell)};x)\Big)\right\| \nonumber\\
=&\left|w(z^{(\ell+1)}, z^{(\ell)})\right|\left\|  h^{(\ell)}\big(\bar{g}^{(\ell)}(z^{(\ell)};x)\big)- h^{(\ell)}\big(g^{(\ell)}(\rho, z^{(\ell)};x)\big)\right\| \nonumber\\
\leq&\left|w(z^{(\ell+1)}, z^{(\ell)})\right|c_0\left\|  \bar{g}^{(\ell)}(z^{(\ell)};x)- g^{(\ell)}(\rho, z^{(\ell)};x)\right\|\nonumber\\
=&\left|w(z^{(\ell+1)}, z^{(\ell)})\right|c_0\left\| \frac{1}{m^{(\ell-1)}}\sum_{j=1}^{m^{(\ell-1)}}w(z^{(\ell)},z^{(\ell-1)}_j)\bar{f}^{(\ell-1)}(z^{(\ell-1)}_j;x)-g^{(\ell)}(\rho, z^{(\ell)};x)\right\|\nonumber\\
\leq& \left|w(z^{(\ell+1)}, z^{(\ell)})\right|c_0\left\| \frac{1}{m^{(\ell-1)}}\sum_{j=1}^{m^{(\ell-1)}}w(z^{(\ell)},z^{(\ell-1)}_j)\Big(\bar{f}^{(\ell-1)}(z^{(\ell-1)}_j;x)-f^{(\ell-1)}(\rho, z^{(\ell-1)}_j;x)\Big)\right\|\nonumber\\
&+\left|w(z^{(\ell+1)}, z^{(\ell)})\right|c_0\left\| \frac{1}{m^{(\ell-1)}}\sum_{j=1}^{m^{(\ell-1)}}w(z^{(\ell)},z^{(\ell-1)}_j)f^{(\ell-1)}(\rho, z^{(\ell-1)}_j;x) - g^{(\ell)}(\rho, z^{(\ell)};x)\right\|\nonumber\\
\leq&\left|w(z^{(\ell+1)}, z^{(\ell)})\right|c_0\frac{1}{m^{(\ell-1)}}\sum_{j=1}^{m^{(\ell-1)}}\left\| w(z^{(\ell)},z^{(\ell-1)}_j)\Big(\bar{f}^{(\ell-1)}(z^{(\ell-1)}_j;x)-f^{(\ell-1)}(\rho, z^{(\ell-1)}_j;x)\Big)\right\|\nonumber\\
&+\left|w(z^{(\ell+1)}, z^{(\ell)})\right|c_0\left\| \frac{1}{m^{(\ell-1)}}\sum_{j=1}^{m^{(\ell-1)}}w(z^{(\ell)},z^{(\ell-1)}_j)f^{(\ell-1)}(\rho, z^{(\ell-1)}_j;x) - g^{(\ell)}(\rho, z^{(\ell)};x)\right\|\nonumber\\
=&\left|w(z^{(\ell+1)}, z^{(\ell)})\right|c_0\frac{1}{m^{(\ell-1)}}\sum_{j=1}^{m^{(\ell-1)}}\Delta_1^{(\ell)}\big(z^{(\ell)},z^{(\ell-1)}_j\big)+\left|w(z^{(\ell+1)}, z^{(\ell)})\right|c_0\Delta_2^{(\ell)}\big(z^{(\ell)}\big)\nonumber
\end{align}

Therefore,
\begin{align}
    &\E_{z^{(1)},\ldots, z^{(\ell)}}\;c_0\Delta_1^{(\ell+1)}\big(z^{(\ell+1)},z^{(\ell)}\big)\nonumber\\
    \leq& \E_{z^{(1)},\ldots, z^{(\ell)}}\;\left|w(z^{(\ell+1)}, z^{(\ell)})\right|c_0^2\frac{1}{m^{(\ell-1)}}\sum_{j=1}^{m^{(\ell-1)}}\Delta_1^{(\ell)}\big(z^{(\ell)},z^{(\ell-1)}_j\big)\nonumber\\
    &+\E_{z^{(1)},\ldots, z^{(\ell)}}\;\left|w(z^{(\ell+1)}, z^{(\ell)})\right|c_0^2\Delta_2^{(\ell)}\big(z^{(\ell)}\big)\nonumber\\
    =&\E_{z^{(1)},\ldots, z^{(\ell)}}\;\left|w(z^{(\ell+1)}, z^{(\ell)})\right|c_0^2\Delta_1^{(\ell)}\big(z^{(\ell)},z^{(\ell-1)}\big)\nonumber\\
    &+\E_{z^{(1)},\ldots, z^{(\ell)}}\;\left|w(z^{(\ell+1)}, z^{(\ell)})\right|c_0^2\Delta_2^{(\ell)}\big(z^{(\ell)}\big)\nonumber\\
    =&\E_{z^{(1)},\ldots, z^{(\ell)}}\;\left|w(z^{(\ell+1)}, z^{(\ell)})\right|c_0^2\Delta_1^{(\ell)}\big(z^{(\ell)},z^{(\ell-1)}\big)\nonumber\\
    &+\E_{z^{(\ell-1)}, z^{(\ell)}}\;\left|w(z^{(\ell+1)}, z^{(\ell)})\right|c_0^2\Delta_2^{(\ell)}\big(z^{(\ell)}\big).\label{eqn:alpha-Delta1-temp-bound}
\end{align}
The last equality holds since the variables $z^{(1)}, \ldots, z^{(\ell-2)}$ are missing in the second item of \eqref{eqn:alpha-Delta1-temp-bound}. And now we can apply Lemma \ref{lemma:Delta-1-2} to estimate $\E_{z^{(1)},\ldots, z^{(\ell)}}\;c_0\Delta_1^{(\ell+1)}\big(z^{(\ell+1)},z^{(\ell)}\big)$ further. To be precise, 
\begin{align}
    &\E_{z^{(1)},\ldots, z^{(\ell)}}\;c_0\Delta_1^{(\ell+1)}\big(z^{(\ell+1)},z^{(\ell)}\big)\nonumber\\
     \leq&\E_{z^{(1)},\ldots, z^{(\ell)}}\;\left|w(z^{(\ell+1)}, z^{(\ell)})\right|c_0^2\Delta_1^{(\ell)}\big(z^{(\ell)},z^{(\ell-1)}\big)\nonumber\\
    &+\E_{z^{(\ell-1)}, z^{(\ell)}}\;\left|w(z^{(\ell+1)}, z^{(\ell)})\right|c_0^2\Delta_2^{(\ell)}\big(z^{(\ell)}\big)\nonumber\\
    \leq& \E_{z^{(1)},\ldots, z^{(\ell)}}\;\left|w(z^{(\ell+1)}, z^{(\ell)})w(z^{(\ell)}, z^{(\ell-1)})\right|c_0^3\Delta_1^{(\ell-1)}\big(z^{(\ell-1)},z^{(\ell-2)}\big)\nonumber\\
    &+ \E_{z^{(\ell-2)},\ldots, z^{(\ell)}}\;\left|w(z^{(\ell+1)}, z^{(\ell)})w(z^{(\ell)}, z^{(\ell-1)})\right|c_0^3\Delta_2^{(\ell-1)}\big(z^{(\ell-1)}\big)\nonumber\\
    &+\E_{z^{(\ell-1)}, z^{(\ell)}}\;\left|w(z^{(\ell+1)}, z^{(\ell)})\right|c_0^2\Delta_2^{(\ell)}\big(z^{(\ell)}\big)\nonumber\\
    \leq & \ldots\nonumber\\
     &\vdots \nonumber\\
    \leq& \sum_{k=2}^{\ell}\E_{z^{(\ell-k+1)},\ldots,z^{(\ell)}} \left|\Pi_{i=\ell-k+3}^{\ell+1}w\big(z^{(i)},z^{(i-1)}\big)\right|c_0^k\Delta_2^{(\ell-k+2)}\big(z^{(\ell-k+2)}\big)\label{eqn:alpha-Delta1-temp-temp-bound}\\
    =& \sum_{k=2}^{\ell}\E_{z^{(\ell-k+1)},\ldots,z^{(\ell)}} c_0^kA(k-1,\ell+1)\Delta_2^{(\ell-k+2)}\big(z^{(\ell-k+2)}\big)\label{eqn:alpha-Delta1-bound}
\end{align}
And the inequality in \eqref{eqn:alpha-Delta1-temp-temp-bound} holds since $\Delta_1^{(2)}(z^{(2)},z^{(1)})\equiv0$.

By combing the results in Eqns.\eqref{eqn:diff-bf-f-bound} and \eqref{eqn:alpha-Delta1-bound}, we can obtain 
\begin{align}
&\E_{z^{(1)},\ldots, z^{(\ell)}}\;\left\|\bar{f}^{(\ell+1)}(z^{(\ell+1)};x)- f^{(\ell+1)}(\rho, z^{(\ell+1)}; x)\right\|\nonumber\\
\leq& \sum_{k=2}^{\ell}\E_{z^{(\ell-k+1)},\ldots,z^{(\ell)}} c_0^kA(k-1,\ell+1)\Delta_2^{(\ell-k+2)}\big(z^{(\ell-k+2)}\big)\nonumber\\
&+\E_{z^{(\ell)}}\;c_0\Delta_2^{(\ell+1)}\big(z^{(\ell+1)}\big)\nonumber\\
=&\sum_{k=1}^{\ell}\E_{z^{(\ell-k+1)},\ldots,z^{(\ell)}} c_0^kA(k-1,\ell+1)\Delta_2^{(\ell-k+2)}\big(z^{(\ell-k+2)}\big).\nonumber
\end{align}

Therefore,
\begin{align}
\lim_{m^{(k)}\rightarrow \infty, k=1,\ldots,\ell}\E_{z^{(1)},\ldots, z^{(\ell)}}\; \left\|\bar{f}^{(\ell+1)}(z^{(\ell+1)};x)-f^{(\ell+1)}(\rho, z^{(\ell+1)};x)\right\|=0.\nonumber
\end{align}
The proof is complete.
\end{proof}
\textbf{Step 4.} In this final step, we prove Theorem \ref{theorem:convergence-discrete-NN} based on Lemma \ref{lemma:convergence-discrete-NN}. 
\begin{proof} of Theorem \ref{theorem:convergence-discrete-NN}:\\
(i) This is a special case of Lemma \ref{lemma:convergence-discrete-NN}, since by the definition, we have
\begin{align}
    \hat{f}^{(k)}_j(x)=\bar{f}^{(k)}(z^{(k)}_j;x).\nonumber
\end{align}
(ii) We notice that $u(\cdot)$ is a $K$-dimensional vector valued function on $\cZ{L}$, it is equivalent to 
\begin{align}
    \lim\limits_{m^{(\ell)}\rightarrow \infty, \ell = 1, ...,L} \E\;\left\|[\hat{f}]_k(x)- [f]_k(\rho, u; x)\right\| =0, k = 1,...,K,\label{eqn:equivalent-form-of-ii}
\end{align}
where $[\hat{f}]_k$ and $[f]_k$ are the $k$-th dimension of the functions $\hat{f}$ and $f$, respectively. 

Let $[u]_k$ to be the $k$-th dimension of $u$, we can rewrite $[\hat{f}]_k$ and $[f]_k$ as
\begin{align}
    [\hat{f}]_k(x)= & \frac{1}{m^{(L)}} \sum_{j=1}^{m^{(L)}} w([u]_k,z^{(L)}_j)\hat{f}^{(L)}_j(x) = \bar{f}^{L+1}([u]_k;x),\nonumber\\
    [f]_k(\rho, u; x)=&\int [\u]_k(z^{(L)}) \ff^{(L)}(\rho,z^{(L)};x) \; d\rho^{(L)}(z^{(L)})\nonumber\\
=&\int w([\u]_k,z^{(L)})\ff^{(L)}(\rho,z^{(L)};x) \; d\rho^{(L)}(z^{(L)}).\nonumber\\
=&h^{(L+1)}\left(\int w([\u]_k,z^{(L)})\ff^{(L)}(\rho,z^{(L)};x) \; d\rho^{(L)}(z^{(L)})\right)\nonumber\\
=&f^{(L+1)}(\rho, [u]_k;x),\nonumber
\end{align}
where $h^{(L+1)}$ be an identity mapping on $\R$. Since $[u]_k \in \cZ{L+1}$, Eqn.\eqref{eqn:equivalent-form-of-ii} is then exactly in the form of Lemma \ref{lemma:convergence-discrete-NN} and therefore (ii) of Theorem \ref{theorem:convergence-discrete-NN} holds.

The proof is complete.
\end{proof}



\section{Variance of Discrete Approximation}
In this section, we prove Theorem \ref{var}. Before giving the detailed proof, we need to give the following definitions first. 
\begin{itemize}
    \item[(1)] We denote $\cI^{(\ell)}$ to be the set consisting of all ordered sequences in the form of $\{k_1, k_2, \dots, k_{\ell} \}$ with   $k_{j}\in [m^{(j)}]$ and $j\in [\ell]$. That is
\begin{align}
    \cI^{(\ell)} := [m^{(1)}] \otimes [m^{(2)}] \otimes \cdots \otimes [m^{(\ell)}],\nonumber
\end{align}
where $\otimes$ means the  Cartesian product.

\item[(2)] We denote $\hat{\mathcal{Z}}^{(\ell)} = \{z^{(\ell)}_{j}:~ j\in[m^{(\ell)}]  \}$, %$\hcZ=\{\hcZ^{(0)},\cdots, \hcZ^{(L)}\}$% 
and let 
\begin{align}
    \{z\}_{\cI^{(\ell)}}=  \hat{\mathcal{Z}}^{(1)}\otimes \cdots \otimes \hat{\mathcal{Z}}^{(\ell)}.\nonumber
\end{align}

\item[(3)] $\EE[f]$ means taking full expectation on all the random variables. $\EE_{\hcZ^{(\ell)}}[f]$ (or $\EE_{\{z\}_{\cI^{(\ell)}}}[f]$) stands for the conditional expectation  on $\hcZ^{(\ell)}$ (or $\{z\}_{\cI^{(\ell)}}$).

\item[(4)] We let $\breve{f}^{(0)}(\rho, z^{(0)};x) = x_{z^{(0)}}$ with $z^{(0)}\in \cZ{0}$. For $z^{(\ell)}\in \cZ{\ell}$ and $\ell\in [L]$, we define 
\begin{align}
\breve{f}^{(\ell)}(\rho, z^{(\ell)};x) =&f^{(\ell)}(\rho,z^{(\ell)};x)+\nabla \hl\big( \gl(\rho,\yh{\zl};x) \big)\left[\breve{g}^{(\ell)}(\rho, z^{(\ell)};x) - \gl(\rho,\zl;x) \right],\label{def bf}
\end{align}
where
\begin{align}
    \breve{g}^{(\ell)}(\rho,z^{(\ell)};x)=\frac{1}{m^{(\ell-1)}} \sum_{i=1}^{m^{(\ell-1)}} w(\zl, \zmi_i)\breve{f}^{(\ell-1)}(\rho,z^{(\ell-1)}_i;x), \mbox{ with } \ell\in [\yh{L}].\nonumber
\end{align}

Moreover, we define 
\begin{eqnarray}\label{ffo}
\breve{f}(\rho,u ; x) = \frac{1}{m^{(L)}}\sum_{i=1}^{m^{(L)}}\breve{f}^{(L)}(\rho,\zL_i;x)u(\zL_i).
\end{eqnarray}
Note that $\breve{f}^{(\ell)}$ and $ \breve{g}^{(\ell)}$  depend on $\{z\}_{\cI^{(\ell-1)}}$ as well, but for  simplicity, we do not show them in the definitions explictly.
 

\item[(5)] We define $S^{(\ell)}(\rho,z^{(1)}, \ldots, z^{(\ell)};x)$ for $\ell = [L]$ by letting
\begin{align}
&S^{(1)}(\rho, z^{(1)};x) =h^{(1)}\left( \frac{1}{d}\sum_{i=1}^d w(z^{(1)}, \yh{z^{(0)}_i}) x_{z^{(0)}_i}\right),\nonumber\\
&S^{(\ell)}(\rho,z^{(1)}, \dots, z^{(\ell)};x)=\hl \big( \gl(\rho,\zl;x) \big) \label{def S}\\
&\quad \quad \quad \quad +\nabla \hl\big(\gl(\rho,\zl;x) \big)\left[ w(\zl, \zmi)S^{(\ell-1)}(\rho, z^{(1)},\ldots, \zmi;x)- \gl(\rho, \zl;x) \right],\nonumber
\end{align}
where $\ell\in\{2, 3,\dots, L\}$. Finally, we define
\begin{align*}
\tilde{S}(\rho,z^{(1)}, \dots, z^{(L)},u;x) = S^{(L)}(\rho,z^{(1)}, \dots, z^{(L)};x)u( z^{(L)}) - f(\rho,u;x).
\end{align*}
We notice that the Assumption \ref{ass:3} is slight stronger than assuming the bounded $q$-th moment on  $\tilde{S}(\rho,z^{(1)}, \dots,  z^{(L)},u;x)$. From the bounded gradient of   Assumption \ref{ass:2}, we will prove that:
\begin{align}
\E_{z^{(1)}, \dots, z^{(L)}} \left\|\tilde{S}(\rho,z^{(1)}, \dots,  z^{(L)},u;x)\right\|^2\leq c_{M_2},\nonumber
\end{align}
where $c_{M_2}$ is a constant, and  $\E\tilde{S}(\rho,z^{(1)}, \dots, z^{(L)},u;x)=0 $.
\end{itemize}

We give the detailed proof of Theorem \ref{var} below:\\
\textbf{step 1.} We prove 
\begin{align}
 \E_{\{z\}_{\cI^{(\ell-1)}}}\breve{f}^{(\ell)}(\rho,\zl_j;x) = f^{(\ell)}(\rho,\zl_j;x), ~~\ell\in [L],\label{stt1}
\end{align} 
and 
$$ \E_{\{z\}_{\cI^{(L)}}}\breve{f}(\rho,u;x) = f(\rho,u;x). $$
\begin{proof}
We prove it by induction. When $\ell=1$, the statement is true. Suppose at $\ell-1$, the statement is true.  We consider $\ell$. For all $j\in [m^{(\ell)}]$, we have
\begin{align}
&\EE_{\{z\}_{\cI^{(\ell-1)}}}\breve{f}^{(\ell)}(\rho,\zl_j;x)\notag\\
=& \EE_{\hcZ^{(\ell-1)}}\left[\EE_{\{z\}_{\cI^{\ell-2}}}\breve{f}^{(\ell)}(\rho,\zl_j;x)\right]\notag\\
\overset{\eqref{def bf}}{=}& \EE_{\hcZ^{(\ell-1)}}\Bigg\{\nabla \hl( \gl(\rho,\zl_j;x) )\Bigg[ \frac{1}{m^{(\ell-1)}} \sum_{i=1}^{m^{(\ell-1)}} w(\zl_j, \zmi_i)\EE_{\{z\}_{\cI^{\ell-2}}}\breve{f}^{(\ell-1)}(\rho,\zmi_i;x)\nonumber\\
&\quad \quad\quad\quad\quad \quad\quad\quad\quad\quad\quad \quad\quad\quad\quad\quad - \gl(\rho,\zl_j;x) \Bigg]\Bigg\}+\EE_{\hcZ^{(\ell-1)}}\left[\hl ( \gl(\rho,\zl_j;x) )\right]\notag\\
\overset{a}=&\hl ( \gl(\rho,\zl_j;x)+ \EE_{\hcZ^{(\ell-1)}}\nabla \hl\big( \gl(\rho,\zl_j;x) \big)\Bigg[ \frac{1}{m^{(\ell-1)}} \sum_{i=1}^{m^{(\ell-1)}} \notag\\
& \quad \quad\quad\quad\quad \quad\quad\quad\quad\quad\quad \quad\quad\quad\quad\quad w(\zl_j, \zmi_i)f^{(\ell-1)}(\rho,\zmi_i;x)- \gl(\rho,\zl_j;x) \Bigg]\notag\\
 \overset{\eqref{eq:nn-layer}}{=}&\hl ( \gl(\rho,\zl_j;x )) \notag\\
\overset{\eqref{eq:nn-activation}}{=}& f^{(\ell)}(\rho,\zl_j;x),\notag
\end{align}
where  $\overset{a}=$ applies \eqref{stt1} on $\ell-1$.
Then 
\begin{align}
\E \breve{f}(\rho,u;x) =& \E_{\{z\}_{\cI^{(L)}}} \frac{1}{m^{(L)}}\sum_{j=1}^{m^{(L)}}\breve{f}^{(L)}(\rho,z_j^{(L)};x) u_j^{(L)} \nonumber\\
=&\E_{\hcZ^{(L)}} \frac{1}{m^{(L)}}\sum_{j=1}^{m^{(L)}}f^{(L)}(\rho,z_j^{(L)};x) u(z^{(L)}_j)\nonumber\\
=& f(\rho,u;x).\nonumber
\end{align}
\end{proof}

\textbf{Step 2.}  In this step, we compute 
\begin{align}
\E\left\| \breve{f}(\rho, u;x)-f(\rho,u;x)\right\|^2.\nonumber
\end{align}
\begin{proof}
We first show that
 \begin{eqnarray}\label{bff1}
 \breve{f}(\rho, u;x)=  \prod_{\ell=1}^L \frac{1}{m^{(\ell)}}\left[\sum_{i\in \cI^{(L)}} S^{(L)}(\rho,z^{(1)}_{i_1}, \dots,z^{(L)}_{i_L};x) u(z^{(L)}_{i_L})\right].
 \end{eqnarray}

Clearly, we have $\breve{f}^{(1)} (\rho,z^{(1)}_j;x) =S^{(1)} (\rho,z^{(1)}_j;x) =f^{(1)} (\rho,z^{(1)}_j;x)$  for all $j\in [m^{(1)}]$.  Then we can  verify that  for all  $j\in  [m^{(2)}]$, 
\begin{align}
\breve{f}^{(2)}(\rho,z^{(2)}_{j};x) = \frac{1}{m^{(1)}} \sum_{i=1}^{m^{(1)}}S^{(2)}(\rho,z^{(1)}_{i}, z^{(2)}_{j};x).\label{ffo0}
\end{align}


We then prove for all $\ell \in \{ 3, \dots, L\}$ and  $j\in [ m^{(\ell)}]$, we have 
\begin{align}
\breve{f}^{(\ell)}(\rho,z^{(\ell)}_{j};x) =  \prod_{k=1}^{\ell-1} \frac{1}{m^{(k)}}\left[ \sum_{i\in\cI^{(\ell-1)}}S^{(\ell)}(\rho,z^{(1)}_{i_1}, \dots,z^{(\ell-1)}_{i_{\ell-1}}, z^{(\ell)}_{j};x)\right]. \label{ffo1}
\end{align}

\yh{[better use $s\in \mathcal{I}^{(l-1)}$ for index?]}

Suppose the above statement is  true at $\ell-1$, then from \eqref{def bf}, we have
\begin{align}
&\breve{f}^{(\ell)}(\rho,\zl_{j};x)\notag\\
 \overset{\eqref{def bf}}=& f^{(\ell)} (\rho,\zl_j;x ) -\nabla \hl( \gl(\rho,\zl_j;x) ) \gl(\rho,\zl_j;x)+ \nabla \hl( \gl(\rho,\zl_j;x) )\times \notag \\
 &\quad\quad\quad\quad\quad\quad\quad\quad\quad\quad\quad\quad\quad\quad\quad\quad \frac{1}{m^{(\ell-1)}} \sum_{i=1}^{m^{(\ell-1)}} w(\zl_j, \zmi_i)\breve{f}^{(\ell-1)}(\rho,\zmi_i;x)\notag\\
 \overset{a}=&f^{(\ell)} (\rho,\zl_j;x )-\nabla \hl( \gl(\rho,\zl_j;x) ) \gl(\rho,\zl_j;x) + \nabla \hl( \gl(\rho,\zl_j;x) )\times \nonumber \\
 &\frac{1}{m^{(\ell-1)}} \sum_{i=1}^{m^{(\ell-1)}}\left[\prod_{k=1}^{\ell-2} \frac{1}{m^{(k)}}\left(\sum_{s\in\cI^{\ell-2}} S^{(\ell-1)}(\rho,z^{(1)}_{s_1}, \dots,z^{(\ell-2)}_{s_{\ell-2}}, z^{(\ell-1)}_i;x)\right)w(\zl_{j}, \zmi_{i})\right]\notag\\
=&f^{(\ell)} (\rho,\zl_j;x )-\nabla \hl( \gl(\rho,\zl_j;x) ) \gl(\rho,\zl_j;x)+\nabla \hl( \gl(\rho,\zl_j;x) ) \times \notag\\ &\quad\quad\quad\quad\quad\quad\quad\quad\quad\prod_{k=1}^{\ell-1} \frac{1}{m^{(k)}}\left[\sum_{s\in\cI^{(\ell-1)}} S^{(\ell-1)}(\rho,z^{(1)}_{s_1}, \dots,z^{(\ell-1)}_{s_{\ell-1}};x)w(\zl_{j}, \zmi_{s_{\ell-1}})\right]\notag\\
 =&  \prod_{k=1}^{\ell-1} \frac{1}{m^{(k)}}\left[\sum_{s\in\cI^{(\ell-1)}} \left(f^{(\ell)} (\rho,\zl_j;x ) -\nabla \hl( \gl(\rho,\zl_j;x) ) \gl(\rho,\zl_j;x)\right)\right] \notag\\
 &+ \nabla \hl( \gl(\rho,\zl_j;x) )\prod_{k=1}^{\ell-1} \frac{1}{m^{(k)}}\left[\sum_{s\in\cI^{(\ell-1)}} S^{(\ell-1)}(\rho,z^{(1)}_{s_1}, \dots,z^{(\ell-1)}_{s_{\ell-1}};x)w(\zl_{j}, \zmi_{s_{\ell-1}})\right]\notag\\
 =&\prod_{k=1}^{\ell-1} \frac{1}{m^{(k)}}\left[ \sum_{s\in\cI^{(\ell-1)}}S^{(\ell)}(\rho,z^{(1)}_{s_1}, \dots,z^{(\ell-1)}_{s_{\ell-1}}, z^{(\ell)}_{j};x)\right],\notag
\end{align}
where in $\overset{a}=$, we use \eqref{ffo1} on $\ell-1$. So we obtain \eqref{ffo1}  on $\ell$.  Then plugging \eqref{ffo1} with $\ell =L$ into \eqref{ffo}, we can obtain \eqref{bff1}. Also by the same technique of Step 1, we can obtain 
\begin{align}
\EE_{z^{(1)}, \dots, z^{(\ell-1)}} S^{(\ell)}(\rho,z^{(1)}, \dots, z^{(\ell)};x) = f^{(\ell)}(\rho,z^{(\ell)};x), ~~\ell\in [L],\label{exp z}
\end{align}
and
\begin{align}
\EE_{z^{(1)}, \dots, z^{(L)}} S^{(L)}(\rho,z^{(1)}, \dots, z^{(L)};x)u( z^{(L)})  = f(\rho, u;x).\label{exp l}
\end{align}
Recall that
\begin{align}
\tilde{S}(\rho,z^{(1)}, \dots, z^{(L)},u;x) = S^{(L)}(\rho,z^{(1)}, \dots, z^{(L)};x)u( z^{(L)}) - f(\rho,u;x),\nonumber
\end{align}
we have $\E_{z^{(1)}, \dots, z^{(L)}}\tilde{S}(\rho,z^{(1)}, \dots, z^{(L)},u;x) = 0$. 

Now we are ready to bound $\E\left\|\breve{f}(\rho,u;x) - f(\rho,u;x)\right\|^2$.
\begin{align}
&\E \left\| \breve{f}(\rho,u;x) - f(\rho,u;x) \right\|^2\label{lin}\\
=&\prod_{\ell=1}^{L}\frac{1}{(m^{(\ell)})^2}\E\left\| \sum_{s\in \cI^{(L)}} \tilde{S}(\rho,z^{(1)}_{s_1}, \dots, z^{(L)}_{s_L},u;x)     \right\|^2\notag\\
=&\prod_{\ell=1}^{L}\frac{1}{(m^{(\ell)})^2}\E \left[ \sum_{s^a\in \cI^{(L)}}\sum_{s^b\in \cI^{(L)}} \tilde{S}^{\top}(\rho,z^{(1)}_{s^a_1}, \dots, z^{(L)}_{s^a_L},u;x) \tilde{S}(\rho,z^{(1)}_{s^b_1}, \dots, z^{(L)}_{s^b_L},u;x)      \right]\notag\\
=&\sum_{s^a\in \cI^{(L)}}\sum_{s^b\in \cI^{(L)}}\left[ \prod_{\ell=1}^{L}\frac{1}{(m^{(\ell)})^2} \E_{z^{(1)}_{s^a_1}, \dots, z^{(L)}_{s^a_L}}\E_{z^{(1)}_{s^b_1}, \dots, z^{(L)}_{s^b_L}}\tilde{S}^{\top}(\rho,z^{(1)}_{s^a_1}, \dots, z^{(L)}_{s^a_L},u;x) \tilde{S}(\rho,z^{(1)}_{s^b_1}, \dots, z^{L}_{s^b_L},u;x) \right]\notag\\
\overset{a}{=}&\sum_{s^a\in \cI^{(L)}}\sum_{s^b\in \cI^{(L)}}\left[ \prod_{\ell=1}^{L}\frac{1}{(m^{(\ell)})^2} \E_{\zl_{s^a_\ell}, \ell\in p^{ab}}\E_{\zl_{s^a_\ell}, \ell\in q^{ab}}\E_{\zl_{s^b_\ell}, \ell\in q^{ab}}\tilde{S}^{\top}(\rho,z^{(1)}_{s^a_1}, \dots, z^{(L)}_{s^a_L},u;x) \tilde{S}(\rho,z^{(1)}_{s^b_1}, \dots, z^{L}_{s^b_L},u;x) \right]\notag\\
\overset{b}{=}&\sum_{s^a\in \cI^{(L)}}\sum_{s^b\in \cI^{(L)}}\left[ \prod_{\ell=1}^{L}\frac{1}{(m^{(\ell)})^2} \E_{\zl_{s^a_\ell}, \ell\in p^{ab}}\left\|\E_{\zl_{s^a_\ell}, \ell\in q^{ab}}\tilde{S}(\rho,z^{(1)}_{s^a_1}, \dots, z^{(L)}_{s^a_L},u;x)\right\|^2  \right]\notag\\
\overset{c}{=}&\sum_{\ell=0}^L \sum_{\mathcal{a}\in \mathcal{C}^\ell}\left[ \Big(\prod_{k\in \mathcal{a}}\frac{1}{m^{(k)}} \prod_{k\in \mathcal{a}^c}\frac{m^{(k)}-1}{m^{(k)}}\Big) \E_{z^{(i)}, i\in \mathcal{a}}\left\|\E_{ z^{(j)}, j\in \mathcal{a}^c}\tilde{S}(\rho,z^{(1)}, \dots, z^{(L)},u;x)\right\|^2  \right]\notag\\
\overset{d}{=}&\sum_{\ell=1}^L \sum_{\mathcal{a}\in \mathcal{C}^\ell}\left[ \Big(\prod_{k\in \mathcal{a}}\frac{1}{m^{(k)}} \prod_{k\in \mathcal{a}^c}\frac{m^{(k)}-1}{m^{(k)}}\Big) \E_{z^{(i)}, i\in \mathcal{a}}\left\|\E_{ z^{(j)}, j\in \mathcal{a}^c}\tilde{S}(\rho,z^{(1)}, \dots, z^{(L)},u;x)\right\|^2  \right].\notag
\end{align}
In $\overset{a}=$, we denote $p^{ab} = \{\ell: s^a_\ell = s^b_\ell, ~ \ell \in [L]\}$ and $q^{ab} = \{\ell: s^a_\ell \neq s^b_\ell, \ell \in [L]\}$. In $\overset{b}=$,  given $\zl_{s^a_\ell}$ with $\ell\in p^{ab}$, $\tilde{S}(\rho,z^{(1)}_{s^a_1}, \dots, z^{(L)}_{s^a_L},u;x)$ and $\tilde{S}(\rho,z^{(1)}_{s^b_1}, \dots, z^{L}_{s^b_L},u;x)$ are independent, so 
\begin{align}
&\E_{\zl_{s^a_\ell}, \ell\in q^{ab}}\E_{\zl_{s^b_\ell}, \ell\in q^{ab}}\tilde{S}^{\top}(\rho,z^{(1)}_{s^a_1}, \dots, z^{(L)}_{s^a_L},u;x) \tilde{S}(\rho,z^{(1)}_{s^b_1}, \dots, z^{L}_{s^b_L},u;x)\notag\\
=& \E_{\zl_{s^a_\ell}, \ell\in q^{ab}}\tilde{S}^{\top}(\rho,z^{(1)}_{s^a_1}, \dots, z^{(L)}_{s^a_L},u;x)\E_{\zl_{s^b_\ell}, \ell\in q^{ab}} \tilde{S}(\rho,z^{(1)}_{s^b_1}, \dots, z^{L}_{s^b_L},u;x) \notag\\
=&    \left\|\E_{\zl_{s^a_\ell}, \ell\in q^{ab}} \tilde{S}(\rho,z^{(1)}_{s^a_1}, \dots, z^{(L)}_{s^a_L},u;x)\right\|^2.\nonumber
\end{align}
In $\overset{c}=$, we denote $\mathcal{C}^\ell$
as the set of all the $\ell$-combinations of $[L]$, specially $\mathcal{C}^0 = \{\varnothing\}$. Then for all $\mathcal{a}\in \mathcal{C}^\ell$, we denote $\mathcal{a}^c = [L]\setminus \mathcal{a}$. We classify $p^{ab}$ into $L+1$ categories,i.e., $\mathcal{C}^\ell$ with $\ell=0,\ldots, L$,  according to their set size.  Then for each $\ell\in [m] $, consider  we sample $2$ numbers from $m^{(\ell)}$ with replacement, There are $m^{(\ell)}$ possibilities if the two numbers are the same and  $m^{(\ell)}(m^{(\ell)}-1)$ possibilities  if the two numbers are different. In $\overset{d}{=}$, we use when $\ell = 0$,  
$$ \E_{ z^{(j)}, j\in \mathcal{a}^c}\tilde{S}(\rho,z^{(1)}, \dots, z^{(L)},u;x) = \E_{ z^{(1)}, \dots, z^{(L)}}\tilde{S}(\rho,z^{(1)}, \dots, z^{(L)},u;x) = 0. $$


In the following, we first bound $\EE_{z^{(1)},\dots, \yh{z^{(L)}}}\| \tilde{S}(\rho, z^{(1)}, \dots, z^{(L)})\|^2$. We  have
\begin{align}
  &\| \tilde{S}(\rho, z^{(1)}, \dots, z^{(L)})\|\notag\\
  \overset{\eqref{def S}}{=}& \Big\|u(z^{(L)})f^{(L)}(\rho,z^{(L)};x) - f(\rho, u;x) +u(z^{(L)}) \nabla h^{(L)}(g^{(L)}(\rho, z^{(L)};x))\times\notag\\
 & \quad\quad\quad\quad\quad\quad\quad\quad \left[w(z^{(L)}, z^{(L-1) }) S^{(L-1)}(\rho,z^{(1)}, \dots, z^{(L-1)};x) - g^{(L)}(\rho, z^{(L)};x)\right]  \Big\|\notag\\
 \leq & \left\|u(z^{(L)})f^{(L)}(\rho,z^{(L)};x) - f(\rho, u;x)\right\|+  \overbrace{\Big| \nabla h^{(L)}(g^{(L)}(\rho, z^{(L)};x))\Big|}^{\leq c_0 \text ~~from~ Assum.~ \ref{ass:2}}\times\notag\\
 & \quad\quad\quad\quad\quad \Big\|u(z^{(L)})\left[w(z^{(L)}, z^{(L-1) }) S^{(L-1)}(\rho,z^{(1)}, \dots, z^{(L-1)};x) - g^{(L)}(\rho, z^{(L)};x)\right]\Big\| \notag\\
\overset{\eqref{def S}}{=}& \left\|u(z^{(L)})f^{(L)}(\rho,z^{(L)};x) - f(\rho, u;x)\right\|\notag\\
 & \quad\quad\quad\quad\quad~~~ +c_0\Big\|u(z^{(L)})\left[w(z^{(L)}, z^{(L-1) }) f^{(L-1)}(\rho, z^{(L-1)};x) - g^{(L)}(\rho, z^{(L)};x)\right]\Big\|\notag\\
 &\quad\quad\quad\quad\quad\quad\quad\quad\quad +c_0\Big\|u(z^{(L)})w(z^{(L)}, z^{(L-1) }) \overbrace{ \nabla h^{(L-1)}(g^{(L-1)}(\rho, z^{(L-1)};x))}^{\leq c_0 \text ~~from~ Assum.~ \ref{ass:2}}\times\notag\\
 &\quad\quad\quad\quad\quad~~~\left[ w(z^{(L-1)}, z^{(L-2) }) S^{(L-2)}(\rho,z^{(1)}, \dots, z^{(L-2)};x) - g^{(L-1)}(\rho, z^{(L-1)};x)\right]\Big\|\notag\\
    \leq & \ldots\nonumber\\
     &\vdots \nonumber\\
\leq&\left\|u(z^{(L)})f^{(L)}(\rho,z^{(L)};x) - f(\rho, u;x)\right\|+  \sum_{\ell=3}^{L}c_o^{L-\ell+1}\notag\\
&\Bigg\|u^{(L)}(z^{(L)})\prod_{i=\ell+1}^{L} \left( w(z^{(i)}, z^{(i-1)})\right) \left[ w(z^{(\ell)}, z^{(\ell-1)})f^{(\ell-1)}(\rho,z^{(\ell-1)};x) -g^{(\ell)}(\rho, z^{(\ell)};x)\right]\Bigg\|\notag\\
&~+c_0^{L-1}\Bigg\|u^{(L)}(z^{(L)})\prod_{i=1}^{L} \left( w(z^{(i)}, z^{(i-1)})\right) \underbrace{\left[w(z^{(2)}, z^{(1)})S^{(1)}(\rho, z^{(1)};x) - g^{(2)}(\rho, z^{(2)};x)\right]}_{S^{(1)}(\rho, z^{(1)};x) = f^{(1)}(\rho, z^{(1)};x)}  \Bigg\|.\notag
\end{align}
We have 
\begin{align}
&\E_{z^{(1)}, \dots, z^{(L)}}\| \tilde{S}(\rho, z^{(1)}, \dots, z^{(L)})\|^2\notag\\
\leq& L\E_{z^{(1)}, \dots, z^{(L)}} \left\|u(z^{(L)})f^{(L)}(\rho,z^{(L)};x) - f(\rho, u;x)\right\|^2+  L\E_{z^{(1)}, \dots, z^{(L)}} \sum_{\ell=2}^{L}c_o^{L-\ell+1}\notag\\
&\quad~ \Bigg\|u^{(L)}(z^{(L)})\prod_{i=\ell+1}^{L} \left( w(z^{(i)}, z^{(i-1)})\right) \left[ w(z^{(\ell)}, z^{(\ell-1)})f^{(\ell-1)}(\rho,z^{(\ell-1)};x) -g^{(\ell)}(\rho, z^{(\ell)};x)\right]\Bigg\|^2\notag\\
%\overset{a}{\leq}& L\E_{z^{(1)}, \dots, z^{(L)}} \left\|u(z^{(L)})f^{(L)}(\rho,z^{(L)};x) - f(\rho, u;x)\right\|^2+  L\Bigg(\E_{z^{(1)}, \dots, z^{(L)}} \sum_{\ell=2}^{L}c_o^{L-\ell+1}\Bigg\|u^{(L)}(z^{(L)})\notag\\
\overset{a}{\leq}& L\E_{z^{(1)}, \dots, z^{(L)}} \left\|u(z^{(L)})f^{(L)}(\rho,z^{(L)};x) - f(\rho, u;x)\right\|^2+  L\yh{\sum_{\ell=2}^{L} c_o^{L-\ell+1}} \Bigg(\E_{z^{(1)}, \dots, z^{(L)}} \Bigg\|u^{(L)}(z^{(L)})\notag\\
&~\prod_{i=\ell+1}^{L} \left( w(z^{(i)}, z^{(i-1)})\right) \left[ w(z^{(\ell)}, z^{(\ell-1)})f^{(\ell-1)}(\rho,z^{(\ell-1)};x) -g^{(\ell)}(\rho, z^{(\ell)};x)\right]\Bigg\|^{2(1+\alpha)^{L}}\Bigg)^{(1+\alpha)^{-L}}\notag\\
%\leq&L c_{M_1} + L (c_{M}\vee 1) \sum_{\ell=2}^{L-1}c_o^{L-\ell+1}. \notag
\leq&L c_{M_1} + L (c_{M}\vee 1) \sum_{\ell=2}^{L-1}c_o^{L-\ell+1}. \notag
\end{align}
where in $\overset{a}\leq$, we use  Jensen Inequality, and in $\overset{b}{\leq}$, we use Assumption \ref{ass:3}, $\|u(z^{(L)}) \|\leq \|u(z^{(L)}) \|\vee 1 $, and $|w(z^{(i)}, z^{(i-1)})|\leq  |w(z^{(i)}, z^{(i-1)})|\vee 1 $ with $i\in \{3, \dots, L \}$.
\begin{align}
&\sum_{\ell=2}^L \sum_{\mathcal{a}\in \mathcal{C}^\ell}\left[ \Big(\prod_{k\in \mathcal{a}}\frac{1}{m^{(k)}} \prod_{k\in \mathcal{a}^c}\frac{m^{(k)}-1}{m^{(k)}}\Big) \E_{z^{(i)}, i\in \mathcal{a}}\left\|\E_{ z^{(j)}, j\in \mathcal{a}^c}\tilde{S}(\rho,z^{(1)}, \dots, z^{(L)},u;x)\right\|^2  \right]\label{ell1s}\\
\yh{\le}&\sum_{\ell=2}^L \sum_{\mathcal{a}\in \mathcal{C}^\ell}\left[ \Big(\prod_{k\in \mathcal{a}}\frac{1}{m^{(k)}} \prod_{k\in \mathcal{a}^c}\frac{m^{(k)}-1}{m^{(k)}}\Big) \E_{z^{(1)}, \dots, z^{(L)}}\left\|\tilde{S}(\rho,z^{(1)}, \dots, z^{(L)},u;x)\right\|^2  \right]\notag\\
=&\mathcal{O} \left(\frac{1}{m^2}\right).\notag
\end{align}
On the other hand, for $\ell=1$, we have
\begin{align}
&\E_{ z^{(L)} }\| \E_{z^{(1)}, \dots, z^{(L-1)} } \tilde{S}(\rho, z^{(1)}, \dots, z^{(L)})\|^2\label{ell3s}\\
  \overset{\eqref{def S} }{=}& E_{ z^{(L)} }\Big\|  u(z^{(L)})f^{(L)}(\rho,z^{(L)};x) - f(\rho, u;x) +u(z^{(L)}) \nabla h^{(L)}(g^{(L)}(\rho, z^{(L)};x))   \E_{z^{(L-1)}}\notag\\
   & \quad\quad\quad\quad \left[w(z^{(L)}, z^{(L-1) }) \E_{z^{(1)}, \dots, z^{(L-2)} } S^{(L-1)}(\rho,z^{(1)}, \dots, z^{(L-1)};x) - g^{(L)}(\rho, z^{(L)};x)\right]  \Big\|^2\notag\\
    \overset{\eqref{exp z}~\& ~\eqref{eq:nn-layer}}{=}& E_{ z^{(L)} }\Big\|  u(z^{(L)})f^{(L)}(\rho,z^{(L)};x) - f(\rho, u;x)\|^2\notag\\
    \overset{a}{\leq}& E_{ z^{(L)} }\Big\|  u(z^{(L)})f^{(L)}(\rho,z^{(L)};x) \Big\|^2,\notag
\end{align}
where $\overset{a}\leq$ uses the fact that $\E\| \tilde{\xi} - \E \tilde{\xi}\|^2\leq\E \|\tilde{\xi} \|^2$ with $\tilde{\xi} =  u(z^{(L)})f^{(L)}(\rho,z^{(L)};x) $.
And for all $j\in [L-1]$,  we have
\begin{align}
    &\E_{ z^{(j)} }\| \E_{z^{(k)}, k\in[L]\setminus\{j\} } \tilde{S}(\rho, z^{(1)}, \dots, z^{(L)})\|^2 \label{ell2s}\\
  \overset{\eqref{def S}}{=}& \E_{ z^{(j)} }\Big\| \underbrace{\E_{z^{(L)}} \left[u(z^{(L)})f^{(L)}(\rho,z^{(L)};x) - f(\rho, u;x)\right]}_{0} +  \E_{z^{(k)}, k\in[L]\setminus\{j\} }\big[u(z^{(L)})   \notag\\
  & \quad\quad~ \nabla h^{(L)}(g^{(L)}(\rho, z^{(L)};x))  \left(w(z^{(L)}, z^{(L-1) }) S^{(L-1)}(\rho,z^{(1)}, \dots, z^{(L-1)};x) - g^{(L)}(\rho, z^{(L)};x)\right) \Big] \Big\|^2\notag\\
  =&\E_{ z^{(j)} } \Big\|-\E_{z^{(L)}}\left[u(z^{(L)})\nabla h^{(L)}(g^{(L)}(\rho, z^{(L)};x)) g^{(L)}(\rho, z^{(L)};x)\right]\notag\\
  & ~+ \E_{z^{(k)}, k\in[L]\setminus\{j\}}\left[u(z^{(L)})\nabla h^{(L)}(g^{(L)}(\rho, z^{(L)};x)) w(z^{(L)}, z^{(L-1) }) S^{(L-1)}(\rho,z^{(1)}, \dots, z^{(L-1)};x)\right] \Big\|^2 \notag\\
   \overset{\eqref{def S}}{=}&\E_{ z^{(j)} } \Big\|-\E_{z^{(L)}}\notag\\
    &~~\Bigg\{u(z^{(L)})\nabla h^{(L)}(g^{(L)}(\rho, z^{(L)};x)) \overbrace{\left[g^{(L)}(\rho, z^{(L)};x)- \E_{z^{(L-1)}}w(z^{(L)}, z^{(L-1) }) f^{(L-1)}(\rho, z^{L-1}; x)\right]}^{0}\Bigg\} \notag\\
  &\quad\quad\quad\quad\quad \quad\quad~+ \E_{z^{(k)}, k\in[L]\setminus\{j\}}\Big\{u(z^{(L)}) \nabla h^{(L)}(g^{(L)}(\rho, z^{(L)};x)) \nabla h^{(L-1)}(g^{(L-1)}(\rho, z^{(L-1)};x))\notag\\ 
 &\quad\quad\quad\quad\quad\quad\quad\quad\quad \quad~~~ \left[w(z^{(L-1)}, z^{(L-2) }) S^{(L-2)}(\rho,z^{(1)}, \dots, z^{(L-2)};x) -g^{(L)}(\rho, z^{(L)};x) \right]\Big\} \Big\|^2 \notag\\
 =& \E_{ z^{(j)} } \Big\|\E_{z^{(k)}, k\in[L]\setminus\{j\}}\Big\{u(z^{(L)}) \nabla h^{(L)}(g^{(L)}(\rho, z^{(L)};x)) w(z^{(L)}, z^{(L-1) }) \nabla h^{(L-1)}(g^{(L-1)}(\rho, z^{(L-1)};x)) \notag\\ 
 &\quad\quad\quad\quad \quad\quad\quad \quad~~~ \left[w(z^{(L-1)}, z^{(L-2) }) S^{(L-2)}(\rho,z^{(1)}, \dots, z^{(L-2)};x) -g^{(L-1)}(\rho, z^{(L-1)};x) \right]\Big\} \Big\|^2 \notag\\
  \leq & \ldots\nonumber\\
     &\vdots \nonumber\\
     =&\E_{ z^{(j)} } \Bigg\|\E_{z^{(k)}, k\in[L]\setminus\{j\}}\Bigg\{u(z^{(L)}) \prod_{k=j+2}^{L}\left[\nabla h^{(k)}(g^{(k)}(\rho, z^{(k)};x))w(z^{(k)}, z^{(k-1) }) \right]\notag\\ 
     & \quad\quad~ \nabla h^{(j+1)}(g^{(j+1)}(\rho, z^{(j+1)};x))\left[w(z^{(j+1)}, z^{(j) }) S^{(j)}(\rho,z^{(1)}, \dots, z^{(j)};x) -g^{(j+1)}(\rho, z^{(j+1)};x) \right]\notag\\
     \overset{\eqref{exp z}}=&\E_{ z^{(j)} } \Bigg\|\E_{z^{(j+1)},\dots, z^{(L)}}\Bigg\{u(z^{(L)}) \prod_{k=j+2}^{L}\left[\nabla h^{(k)}(g^{(k)}(\rho, z^{(k)};x))w(z^{(k)}, z^{(k-1) }) \right]\notag\\ 
     & \quad\quad\quad\quad~~   \nabla h^{(j+1)}(g^{(j+1)}(\rho, z^{(j+1)};x))\underbrace{\left[w(z^{(j+1)}, z^{(j) }) f^{(j)}(\rho, z^{(j)};x) -g^{(j+1)}(\rho, z^{(j+1)};x)\right]}_{\E_{z^{(j)}}w(z^{(j+1)}, z^{(j) }) f^{(j)}(\rho, z^{(j)};x) =g^{(j+1)}(\rho, z^{(j+1)};x)} \Bigg\}\Bigg\|^2\notag\\
     \leq&\E_{ z^{(j)} } \Bigg\|\E_{z^{(j\yh{+1})},\dots, z^{(L)}}\Bigg\{u(z^{(L)}) \prod_{k=j+2}^{L}\left[\nabla h^{(\yh{k})}(g^{(\yh{k})}(\rho, z^{(\yh{k})};x))w(z^{(k)}, z^{(k-1) }) \right]\notag\\ 
     & \quad\quad \quad\quad\quad\quad\quad\quad\quad\quad\quad\quad\quad~~ \nabla h^{(j+1)}(g^{(j+1)}(\rho, z^{(j+1)};x))\left[w(z^{(j+1)}, z^{(j) }) f^{(j)}(\rho, z^{(j)};x) \right]\Bigg\}\Bigg\|^2\notag\\
     =&\E_{z^{(j)}}\left\| \E_{z^{(j+1)}} f^{(j)}(\rho,z^{(j)};x) \frac{\partial f(\rho,u;x)}{\partial z^{(j+1)}}  w(z^{(j+1)}, z^{(j)}) \right\|^2.\notag
\end{align} 
Plugging \eqref{ell1s}, \eqref{ell3s}, and \eqref{ell2s} into \eqref{lin}, we have
\begin{align}
    &\E \left\| \breve{f}(\rho,u;x) - f(\rho,u;x) \right\|^2\notag\\
    \leq& \sum_{\ell=1}^{L-1} \E_{z^{(\ell)}}\left\| \E_{z^{(\ell+1)}} f^{(\ell)}(\rho,z^{(\ell)};x) \frac{\partial f(\rho,u;x)}{\partial z^{(\ell+1)}}  w(z^{(\ell+1)}, z^{(\ell)}) \right\|^2 \notag\\
    &\quad\quad\quad\quad\quad~  +\E_{ z^{(L)} }\Big\|  u(z^{(L)})f^{(L)}(\rho,z^{(L)};x) \Big\|^2 + \mathcal{O}\left(\frac{1}{m^2}\right)\notag.
\end{align}
\end{proof}


\textbf{Step 3.} Now the remaining to do is to bound
$$\E\left\| \breve{f}(\rho,u;x)-\hf(x)\right\|^2,    $$
which is carried out in this step.  
\begin{proof}
We denote 
 $$
\bbu(z^{(L)})= 
\begin{cases}
\|u(z^{(L)})\|,&   \|u(z^{(L)}) \|\geq 1,\\
1,&   \text{otherwise}, \\
\end{cases}
$$
for all $z^{(L)}\in \mathcal{Z}^{(L)}$, and 
 $$
\bbw(z^{(\ell)}, z^{(\ell-1)})= 
\begin{cases}
|w(z^{(\ell)}, z^{(\ell-1)})|,&   |w(z^{(\ell)}, z^{(\ell-1)})|\geq 1,\\
1,&   \text{otherwise}, \\
\end{cases},
$$
for all $z^{(\ell)}\in \mathcal{Z}^{(\ell)}$ and  $\ell \in [L]$. We  denote $\cA^{(\ell)}$ to be
\begin{align} \cA^{(\ell)} = [m^{(\ell)}] \otimes [m^{(\ell+1)}] \otimes \cdots \otimes [m^{(L)}].\nonumber
\end{align}
 Then, for $\ell \in \{2, \cdots, L \}$ and  $\ts\in \cA^{(\ell-1)}$,  we define
 \begin{align}
 \Psi^{(\ell)}(\ts) = \bbu(z^{(L)}_{\ts_L})  \left(\prod_{i = \ell\yh{+1}}^{L} \bbw(z^{(i)}_{\ts_i}, z^{(i-1)}_{\ts_{i-1}})\right),\nonumber
 \end{align}
 and when $\ell=L+1$, we let
 \begin{align}
     \Psi^{(L+1)}(\ts) = \bbu(z^{(L)}_{\ts_L}), ~~ \ts\in \cA^{(L)},\nonumber
 \end{align}
 where for the sake of simplicity, $\ts_{i}$ is the value of the $(i-\ell+1)$-th dimension of $\ts$ with $i=\ell,\ldots,L$.
 
 
For for $\ell\in \{2, 3, \dots, L\}$, and $t\geq0$,  by setting $\beta_t= (1+\alpha)^{t}\geq 1$ with $t\in \{0, \dots, L\}$, we first consider bounding
$$
\EE\sum_{\ts\in \cA^{(\ell)}}  \Big(\prod_{i=\ell}^L \frac{1}{m^{(i)}}\Big) \left| 
\Psi^{(\ell+1)}(\ts)\frac{1}{m^{(\ell-1)}}\sum_{j=1}^{m^{(\ell-1)}}\left[ w(\zl_{\ts_{\ell}},\zmi_{j} )
\breve{f}^{(\ell-1)}(\rho,\zmi_{j};x) -  g^{(\ell)}(\rho,\zl_{\ts_{\ell}};x)\right] \right|^{2\beta_t}.
$$


When $\ell=1$, \eqref{l use} equals to $0$.  When $\ell\geq 2$, from  \eqref{ffo0} and \eqref{ffo1}, we have
\begin{align}
&\EE\sum_{\ts\in \cA^{(\ell)}}  \Big(\prod_{i=\ell}^L \frac{1}{m^{(i)}}\Big) \Bigg| 
\Psi^{(\ell+1)}(\ts)\frac{1}{m^{(\ell-1)}}\sum_{j=1}^{m^{(\ell-1)}}\left[ w(\zl_{\ts_{\ell}},\zmi_{j} )
\breve{f}^{(\ell-1)}(\rho,\zmi_{j};x) -  g^{(\ell)}(\rho,\zl_{\ts_{\ell}};x)\right]     \Bigg|^{2\beta_t}\notag\\
=&
\prod_{i=\ell}^L \frac{1}{m^{(i)}}\EE\sum_{\ts\in \cA^{(\ell)}} \Bigg|  \prod^{\ell-1}_{j=1}\frac{1}{m^{(j)}}\Psi^{(\ell+1)}(\ts)\sum_{\hs\in \cI^{(\ell-2)}}\sum_{j=1}^{m^{(\ell-1)}}\notag\\
&\quad\quad\quad\quad\quad\quad\quad\quad\quad\quad\quad
\bigg[w(z^{(\ell)}_{\ts_{\ell}}, z^{(\ell-1)}_j)S^{(\ell-1)}(\rho,z^{(1)}_{\hs_1}, \dots, z^{(\ell-2)}_{\hs_\ell-2}, \zmi_{j};x) - g^{(\ell)}(\rho,\zl_{\ts_{\ell}};x)\bigg] \Bigg|^{2\beta_t}\notag\\
\overset{a}=&
\prod^{\ell-1}_{j=1}\frac{1}{(m^{(j)})^{2\beta_t}} 
\EE_{z^{(\ell)}, \dots, z^{(L)}}\E_{\{z\}_{\cI^{(\ell-1)}}}\Bigg|  \bbu(z^{(L)}) \prod_{i = \ell+1}^{L} \bbw(z^{(i)}, z^{(i-1)})\sum_{\hs\in \cI^{(\ell-1)}} \notag\\
&\quad\quad\quad\quad\quad\quad\quad\quad\quad\quad\quad\quad\quad\quad\bigg[w(z^{(\ell)}, z^{(\ell-1)}_{\hs_{\ell-1}})S^{(\ell-1)}(\rho,z^{(1)}_{\hs_1}, \dots, z^{(\ell-1)}_{\hs_{\ell-1}};x) - g^{(\ell)}(\rho,\zl;x)\bigg] \Bigg|^{2\beta_t}\notag\\
\overset{b}{=}&\prod^{\ell-1}_{j=1}\frac{1}{(m^{(j)})^{2\beta_t}}\EE_{z^{(\ell)}, \dots, z^{(L)}} \E_{\{z\}_{\cI^{(\ell-1)}}}\left|\sum_{\hs\in \cI^{(\ell-1)}}  \left[\bar{S}^{(\ell)}(\rho,z^{(1)}_{\hs_1}, \dots, z^{(\ell-1)}_{\hs_{\ell-1}},u;x)\right] \right|^{2\beta_t}\notag\\
\overset{c}{=}&\EE_{z^{(\ell)}, \dots, z^{(L)}}\E_{\{z\}_{\cI^{(\ell-1)}}}\left| \prod^{\ell-1}_{j=1}\frac{1}{(m^{(j)})}\sum_{\dot{s}\in\mathcal{B}^{\ell-1}}\sum_{k=1}^{m^{(J^{(\ell)})}}  \left[\bar{S}^{(\ell)}(\rho,z^{(1)}_{\dot{s}^{+k}_1}, \dots,   z^{(\ell-1)}_{\dot{s}^{+k}_{\ell-1}},u;x)\right] \right|^{2\beta_t}\notag\\
\overset{d}{\leq}&  \EE_{z^{(\ell)}, \dots, z^{(L)}} \E_{\{z\}_{\cI^{(\ell-1)}}}  \prod^{J^{(\ell)}-1}_{j=1}\frac{1}{(m^{(j)})}\prod^{\ell-1}_{j=J^{(\ell)}+1}\frac{1}{(m^{(j)})} \sum_{\dot{s}\in\mathcal{B}^{\ell-1}}\notag\\
&\quad\quad\quad\quad\quad\quad\quad\quad\quad\quad\quad\quad\quad\quad\quad\quad\quad\quad\quad\quad\left| \frac{1}{(m^{(J^{(\ell)})})}\sum_{k=1}^{m^{(J^{(\ell)})}}  \left[\bar{S}^{(\ell)}(\rho,z^{(1)}_{\dot{s}^{+k}_1}, \dots,   z^{(\ell-1)}_{\dot{s}^{+k}_{\ell-1}},u;x)\right] \right|^{2\beta_t} \notag\\
\overset{e}{=}&    \EE_{z^{(\ell)}, \dots, z^{(L)}} \E_{\{z\}_{s^{+k}_1, k\in \left[m^{(J^{(\ell)})}\right]}}  \left| \frac{1}{(m^{(J^{(\ell)})})}\sum_{k=1}^{m^{(J^{(\ell)})}}  \left[\bar{S}^{(\ell)}(\rho,z^{(1)}_{s^{+k}_1}, \dots,   z^{(\ell-1)}_{s^{+k}_{\ell-1}},u;x)\right] \right|^{2\beta_t}
\notag\\
\overset{f}{\leq}&\frac{1}{(m^{(J^{(\ell)})})^{2\beta_t}}\EE_{z^{(\ell)}, \dots, z^{(L)}} C^1_{\beta_t}\left[ m^{(J^{(\ell)})}\E_{z^{(1)}, \dots, z^{(\ell-1)}}\left| \bar{S}^{(\ell)}(\rho,z^{(1)}, \dots, z^{(\ell-1)},u;x) \right|^{2\beta_t}  \right]\notag\\
&+ \frac{1}{(m^{(J^{(\ell)})})^{2\beta_t}}\EE_{z^{(\ell)}, \dots, z^{(L)}} C^2_{\beta_t}\left[ m^{(J^{(\ell)})}\E_{z^{(1)}, \dots, z^{(\ell-1)}}\left| \bar{S}^{(\ell)}(\rho,z^{(1)}, \dots, z^{(\ell-1)},u;x) \right|^2  \right]^{\beta_t}\notag\\
\overset{g}{\leq}&  C^0_{\beta_t}\frac{1}{(m^{(J^{(\ell)})})^{\beta_t}}\E_{z^{(1)}, \dots, z^{(L)}}\left|\bar{S}^{(\ell)}(\rho,z^{(1)}, \dots, z^{\ell-1)},u;x)\right|^{2\beta_t}\notag\\
\overset{h}{\leq}& C^0_{\beta_t} (c_{M}\vee 1)\frac{1}{(m^{(J^{(\ell)})})^{\beta_t}}. \label{l use} 
\end{align}
We explain \eqref{l use}. In $\overset{a}=$, we take expectation on $\{z\}_{\cA^\ell}$. In $\overset{b}=$, we denote
$$ \bar{S}^{(\ell)}(\rho,z^{(1)}_{\hs_1}, \dots, z^{(\ell-1)}_{_{\hs_{\ell-1}}};x) =  \bbu(z^{(L)}) \prod_{i = \ell+1}^{L} \bbw(z^{(i)}, z^{(i-1)})\left[w(z^{(\ell)}, z^{(\ell-1)}_{\hs_{\ell-1}})S^{(\ell-1)}(z^{(1)}_{\hs_1}, \dots, z^{(\ell-1)}_{\hs_{\ell-1}}) - g^{(\ell)}(\zl)\right]. $$
In $\overset{c}=$,  we set $$J^{(t)} =\argmin_{t\in[\ell-1]} m^{(t)}$$
and $$\mathcal{B}^{(\ell-1)} = [m^{(1)} ] \otimes \cdots \otimes [m^{(J^{(\ell)}-1)}]\otimes [m^{(J^{(\ell)}+1)}]\cdots\otimes [m^{(\ell-1)}].$$
For any $\dot{s}\in \mathcal{B}^{\ell-1}$ and $k\in [J^{(\ell)}]$, denote the ordered list $\dot{s}^{+k}$ as
 $$
\dot{s}^{+k}_i= 
\begin{cases}
(\dot{s}_{i}+k)\%m^{(i)}+1,&   i\in [J^{(\ell)-1}],\\
k,&   i= J^{(\ell)} , \\
(\dot{s}_{i}+k)\%m^{(i)}+1,&   i\in [L]\setminus[J^{(\ell)}],
\end{cases}
$$
then we can split
$$  
\sum_{\hs\in \cI^{(\ell-1)}} \bar{S}^{(\ell)}(\rho,z^{(1)}_{\hs_1}, \dots, z^{(\ell-1)}_{\hs_{\ell-1}},u;x)
$$
into $|\mathcal{B}^{(\ell-1)}|$ groups with each group containing $m^{(J^{(\ell)})}$ terms. That is 
$$\sum_{\hs\in \cI^{(\ell-1)}} \bar{S}^{(\ell)}(\rho,z^{(1)}_{\hs_1}, \dots, z^{(\ell-1)}_{\hs_{\ell-1}},u;x) =  \sum_{\dot{s}\in\mathcal{B}^{\ell-1}}\sum_{k=1}^{m^{(J^{(\ell)})}}  \left[\bar{S}^{(\ell)}(\rho,z^{(1)}_{\dot{s}^{+k}_1}, \dots,   z^{(\ell-1)}_{\dot{s}^{+k}_{\ell-1}},u;x)\right].  $$
In $\overset{d}\leq$ we use Jensen Inequality, 
$$ \left|\frac{1}{m}\sum_{i=1}^m x_i \right|^p \leq  \frac{1}{m}\sum_{i=1}^m \left|x_i\right|^p, ~~ p\geq 1.   $$
In $\overset{e}=$, we take expectation on all $\{z\}_{\mathcal{B}^{\ell-1}}$ and denote the ordered list $s^{+k}$ as
 $$
s^{+k}= 
\begin{cases}
(1+k)\%m^{(i)}+1,&   i\in [J^{(\ell)-1}],\\
k,&   i= J^{(\ell)} , \\
(1+k)\%m^{(i)}+1,&   i\in [L]\setminus[J^{(\ell)}].
\end{cases}
$$
In $\overset{f}=$, we use
all $\bar{S}^{(\ell)}(\rho,z^{(1)}_{s^{+k}_1}, \dots, z^{(L)}_{s^{+k}_L};x)$ with $k\in m^{(J^{(\ell)})}$are independent  given $\{z^{(\ell)}, \dots, z^{(L)}\}$ (all the indexes are different) and is obtained by Rosenthal Inequality (Refer to Lemma \ref{rosenthal}).  In $\overset{g}=$, we use Jensen inequality,   given $\{z^{(\ell)}, \dots, z^{(L)}\}$,  we have
\begin{align}
\left[\E_{z^{(1)}, \dots, z^{\ell-1}}\left| \bar{S}^{(\ell)}(\rho,z^{(1)}, \dots, z^{(\ell-1)};x)   \right|^2\right]^{\beta_t} \leq  \E_{z^{(1)}, \dots, z^{\ell-1}}\left| \bar{S}^{(\ell)}(\rho,z^{(1)}, \dots, z^{(\ell-1)};x)\right|^{2\beta_t},\nonumber
\end{align}
and 
\begin{align}
    \frac{1}{(m^{(J^{(\ell)})})^{2\beta_t-1}} \leq \frac{1}{(m^{(J^{(\ell)}})^{\beta_t}},\nonumber
\end{align}
since $\beta_t\geq1$. The inequality $\overset{h}\leq$ comes from Assumption \ref{ass:3}, we have
\begin{align}
    &\E_{z^{(1)}, \dots, z^{(L)}}\left|\bar{S}^{(\ell)}(\rho,z^{(1)}, \dots, z^{\ell-1)},u;x)\right|^{2\beta_t}\notag\\ \overset{t\leq L}{\leq}& \left(\E_{z^{(1)}, \dots, z^{(L)}}\left|\bar{S}^{(\ell)}(\rho,z^{(1)}, \dots, z^{\ell-1)},u;x)\right|^{2\beta_L}\right)^{\frac{\beta_t}{\beta_L}}  \notag\\
    =&(c_{M})^{\frac{\beta_t}{\beta_L}}\notag\\
    \leq& c_{M}\vee 1.
\end{align}


On the other hand,  for any $\ell\in \{2, \dots, L\}$ and $j\in [m^{(\ell)}]$, from Lemma \ref{lip}, we have
\begin{align}
&\left|\hf_j^{(\ell)}(x)  -  \hl(\gl(\rho,\zl_j;x)) - \nabla  \hl(\gl(\rho,\zl_j;x))\left[\hat{g}^{(\ell)}_j(x) -  \gl(\rho,\zl_j;x) \right]    \right|\notag\\
& \quad\quad\quad\quad\quad\quad\quad\quad\quad\quad\quad \leq c_1\left| \frac{1}{m^{(\ell-1)}}\sum_{i=1}^{m^{(\ell-1)}} w(\zl_j, \zmi_i)\hf_i^{(\ell-1)}(x) -  \gl(\rho,\zl_j;x)     \right|^{1+\alpha}.\label{tmt}
\end{align}
Denote 
$$\tPsi_s(z^{(\ell)}) = \Psi^{(\ell+2)}(s)\bbw(z^{\ell+1}_{s_{\ell+1}}, \zl),  ~~ \ell \in \{2, \dots, L-1 \},~ s\in \cA^{(\ell+1)}.$$ And let $\cA^{(L+1)} = \{1\}$, denote
$$\tPsi_s(z^{(L)}) = \bbu(z^{(L)}),~~ s\in \cA^{(L+1)}.$$ We have for all $\ell \in \{2, \dots, L\}$,
\begin{align}
&\left|\frac{1}{m^{(\ell)}} \sum^{m^{(\ell)}}_{j=1}\tPsi_s(\zl_j)\left|\hf^{(\ell)}_j(x) - \breve{f}^{(\ell)}(\rho,\zl_j;x)\right|\right|\label{onet}\\
\leq&\frac{1}{m^{(\ell)}}\sum^{m^{(\ell)}}_{j=1}\left|\tPsi_s(\zl_j)\right|\left| \hf^{(\ell)}_j(x) - \breve{f}^{(\ell)}(\rho,\zl_j;x)\right|\notag\notag\\
=& \frac{1}{m^{(\ell)}}\sum^{m^{(\ell)}}_{j=1}\left|\tPsi_s(\zl_j)\right|\times\notag\\
& \quad\quad\quad\left|\hf_j^{(\ell)}(x)  -  \hl(\gl(\rho,\zl_j;x)) - \nabla  \hl(\gl(\rho,\zl_j;x))\left[  \hat{g}^{(\ell)}_j(x)-  \gl(\rho,\zl_j;x) \right]    \right|\notag\\
&+ \frac{1}{m^{(\ell)}}\sum^{m^{(\ell)}}_{j=1}\left|\tPsi_s(\zl_j)\right|\times\notag \\
&\left|\breve{f}^{(\ell)}(\rho,\zl_j;x)  -  \hl(\gl(\rho,\zl_j;x)) - \nabla  \hl(\gl(\rho,\zl_j;x))\left[ \hat{g}^{(\ell)}_j(x) -  \gl(\rho,\zl_j;x) \right]   \right|\notag\\
\overset{a}{\leq}&\frac{c_1}{m^{(\ell)}}\sum^{m^{(\ell)}}_{j=1}\left|\tPsi_s(\zl_j)\right|\left| \frac{1}{m^{(\ell-1)}}\sum_{i=1}^{m^{(\ell-1)}} w(\zl_j, \zmi_i)\hf^{(\ell-1)}_i(x) -  \gl(\rho,\zl_j;x)     \right|^{1+\alpha}\notag\\
&+\frac{1}{m^{(\ell)}}\sum^{m^{(\ell)}}_{j=1}\left|\tPsi_s(\zl_j)\right|\times \notag\\
&\quad\quad~~~\left| \nabla  \hl(\gl(\rho,\zl_j;x)  \frac{1}{m^{(\ell-1)}}\sum_{i=1}^{m^{(\ell-1)}} w(\zl_j, \zmi_i)\Big[\hf^{(\ell-1)}_i(x) -  \breve{f}^{(\ell-1)}(\rho,\zmi_i;x)\Big]   \right|\notag\\
\overset{b}{\leq}&\frac{c_1}{m^{(\ell)}}\sum^{m^{(\ell)}}_{j=1}\left|\tPsi_s(\zl_j) \frac{1}{m^{(\ell-1)}}\sum_{i=1}^{m^{(\ell-1)}}\left[ w(\zl_j, \zmi_i)\hf_i^{(\ell-1)}(x) -  \gl(\rho,\zl_j;x) \right]    \right|^{1+\alpha}\notag\\
&\quad~~~ +\frac{c_0}{m^{(\ell)}}\sum^{m^{(\ell)}}_{j=1}\left|\tPsi_s(\zl_j) \frac{1}{m^{(\ell-1)}}\sum_{i=1}^{m^{(\ell-1)}} w(\zl_j, \zmi_i)\left[\hf^{(\ell-1)}_i(x) -  \breve{f}^{(\ell-1)}(\rho,\zmi_i;x)\right]  \right|, \\
\leq&\frac{c_1}{m^{(\ell)}}\sum^{m^{(\ell)}}_{j=1}\left|\tPsi_s(\zl_j) \frac{1}{m^{(\ell-1)}}\sum_{i=1}^{m^{(\ell-1)}}\left[ w(\zl_j, \zmi_i)\hf_i^{(\ell-1)}(x) -  \gl(\rho,\zl_j;x) \right]    \right|^{1+\alpha}\notag\\
&\quad~~~ +\frac{c_0}{m^{(\ell)}}\sum^{m^{(\ell)}}_{j=1}\left|\tPsi_s(\zl_j) \frac{1}{m^{(\ell-1)}}\sum_{i=1}^{m^{(\ell-1)}} \bbw(\zl_j, \zmi_i)\left|\hf^{(\ell-1)}_i(x) -  \breve{f}^{(\ell-1)}(\rho,\zmi_i;x)\right|  \right|, \notag
\end{align}
where  $\overset{a}\leq$ uses \eqref{tmt} and  $\overset{b}\leq$ uses Assumption \ref{ass:2} and $\| \tPsi_s(\zl_j)\|\geq 1$.
Furthermore, for the first term on the right hand side of \eqref{onet},  we have
\begin{align}
&\left|\tPsi_s(\zl_j) \frac{1}{m^{(\ell-1)}}\sum_{i=1}^{m^{(\ell-1)}} \left[w(\zl_j, \zmi_i)\hf_i^{(\ell-1)}(x) -  \gl(\rho,\zl_j;x) \right]    \right|\notag\\
\leq&  \left| \tPsi_s(\zl_j)  \frac{1}{m^{(\ell-1)}}\sum_{i=1}^{m^{(\ell-1)}} w(\zl_j, \zmi_i)\left[\hf_i^{(\ell-1)}(x) - \breve{f}^{(\ell-1)}(\rho,\zmi_i;x) \right]    \right|\notag\\
&\quad\quad\quad\quad~ +\left| \tPsi_s(\zl_j) \frac{1}{m^{(\ell-1)}}\sum_{i=1}^{m^{(\ell-1)}} \left[w(\zl_j, \zmi_i)\breve{f}^{(\ell-1)}(\rho,\zmi_i;x) -  \gl(\rho,\zl_j;x)   \right] \right|\\
\leq&  \left| \tPsi_s(\zl_j)  \frac{1}{m^{(\ell-1)}}\sum_{i=1}^{m^{(\ell-1)}} \bbw(\zl_j, \zmi_i)\left|\hf_i^{(\ell-1)}(x) - \breve{f}^{(\ell-1)}(\rho,\zmi_i;x) \right|    \right|\notag\\
&\quad\quad\quad\quad~ +\left| \tPsi_s(\zl_j) \frac{1}{m^{(\ell-1)}}\sum_{i=1}^{m^{(\ell-1)}} \left[w(\zl_j, \zmi_i)\breve{f}^{(\ell-1)}(\rho,\zmi_i;x) -  \gl(\rho,\zl_j;x)   \right] \right|.\notag
\end{align}
From Lemma \ref{jcon}, we have
\begin{align}
&\left|\tPsi_s(\zl_j)  \frac{1}{m^{(\ell-1)}}\sum_{i=1}^{m^{(\ell-1)}} \left[w(\zl_j, \zmi_i)\hf_i^{(\ell-1)}(x) -  \gl(\rho,\zl_j;x) \right]    \right|^{1+\alpha}\label{onea}\\
\leq&  (1-q_0)^{-\alpha}\left| \tPsi_s(\zl_j) \frac{1}{m^{(\ell-1)}}\sum_{i=1}^{m^{(\ell-1)}} \bbw(\zl_j, \zmi_i)\Big|\hf_i^{(\ell-1)}(x) - \breve{f}^{(\ell-1)}(\rho,\zmi_i;x) \Big|    \right|^{1+\alpha}\notag\\
&+q_0^{-\alpha}\left| \tPsi_s(\zl_j)  \frac{1}{m^{(\ell-1)}}\sum_{i=1}^{m^{(\ell-1)}}  \left[w(\zl_j, \zmi_i)\breve{f}^{(\ell-1)}(\rho,\zmi_i;x) -  \gl(\rho,\zl_j;x)\right]     \right|^{1+\alpha},\notag
\end{align}
where we simply set  $q_0 = \frac{3}{4}$. 

Plugging \eqref{onea} into \eqref{onet}, we have for for all $\ell\in \{2, \dots, L\}$ and $s\in \cA^{(\ell+1)}$, 
\begin{align}
&\left|\frac{1}{m^{(\ell)}} \sum^{m^{(\ell)}}_{j=1}\tPsi_s(\zl_j)\left|\hf_j^{(\ell)}(x) - \breve{f}^{(\ell)}(\rho,\zl_j;x)\right|\right|\notag\\
\leq&c_1(1-q_0)^{-\alpha}\frac{1}{m^{(\ell)}}\sum_{j=1}^{m^{(\ell)}}\left| \tPsi_s(\zl_j)  \frac{1}{m^{(\ell-1)}}\sum_{i=1}^{m^{(\ell-1)}} \bbw(\zl_j, \zmi_i)\left|\hf_i^{(\ell-1)}(x) - \breve{f}^{(\ell-1)}(\rho,\zmi_i;x) \right|    \right|^{1+\alpha}\notag\\
&+c_1 q_0^{-\alpha}\frac{1}{m^{(\ell)}}\sum_{j=1}^{m^{(\ell)}}\left| \tPsi_s(\zl_j)  \frac{1}{m^{(\ell-1)}}\sum_{i=1}^{m^{(\ell-1)}} \left[w(\zl_j, \zmi_i)\breve{f}^{(\ell-1)}(\rho,\zmi_i;x) -  \gl(\rho,\zl_j;x)\right]     \right|^{1+\alpha}\notag\\
&\quad\quad\quad\quad~ + \frac{c_0}{m^{(\ell)}}\sum_{j=1}^{m^{(\ell)}}\left|\tPsi_s(\zl_j)   \frac{1}{m^{(\ell-1)}}\sum_{i=1}^{m^{(\ell-1)}} \bbw(\zl_{j}, \zmi_i)\left|\hf_i^{(\ell-1)}(x) -  \breve{f}^{(\ell-1)}(\rho,\zmi_i;x)\right|   \right|.\notag
\end{align}
Finally using  Lemma \ref{jcon} again, for all $\ell\in \{2, \dots, L\}$ and $s\in \cA^{(\ell+1)}$,  we obtain
\begin{align}
&\left|\frac{1}{m^{(\ell)}} \sum^{m^{(\ell)}}_{j=1}\tPsi_s(\zl_j)\left|\hf_j^{(\ell)}(x) - \breve{f}^{(\ell)}(\rho,\zl_j;x)\right|\right|^{2\beta_t}\label{ttend}\\
\leq&c_1^{2\beta_t}q_1^{-2\alpha\beta_t-2\beta_t +1}\times\notag\\
&\quad~~ \left(\frac{1}{m^{(\ell)}}\sum_{j=1}^{m^{(\ell)}}\left| \tPsi_s(\zl_j)  \frac{1}{m^{(\ell-1)}}\sum_{i=1}^{m^{(\ell-1)}} \bbw(\zl_j, \zmi_i)\left|\hf_i^{(\ell-1)}(x) - \breve{f}^{(\ell-1)}(\rho,\zmi_i;x) \right|    \right|^{1+\alpha}\right)^{2\beta_t}\notag\\
&+c_1^{2\beta_t}q_0^{-2\alpha\beta_t}(1-q_1)^{-2\beta_t +1}\times\notag\\
&\left(\frac{1}{m^{(\ell)}}\sum_{j=1}^{m^{(\ell)}}\left| \tPsi_s(\zl_j)  \frac{1}{m^{(\ell-1)}}\sum_{i=1}^{m^{(\ell-1)}} \left[w(\zl_j, \zmi_i)\breve{f}^{(\ell-1)}(\rho,\zmi_i;x) -  \gl(\rho,\zl_j;x)  \right]   \right|^{1+\alpha}\right)^{2\beta_t}\notag\\
&+ c_0^{2\beta_t}q_1^{-2\beta_t +1}\times\notag\\
&\quad\quad\quad~~\left(\frac{1}{m^{(\ell)}}\sum_{j=1}^{m^{(\ell)}}\left|\tPsi_s(\zl_j) \frac{1}{m^{(\ell-1)}}\sum_{i=1}^{m^{(\ell-1)}} \bbw(\zl_{j}, \zmi_i)\Big|\hf_i^{(\ell-1)}(x) -  \breve{f}^{(\ell-1)}(\rho,\zmi_i;x)\Big|  \right|\right)^{2\beta_t}\notag\\
\overset{a}{\leq}&c_1^{2\beta_t}q_1^{-2\alpha\beta_t-2\beta_t +1}\times\notag\\
&\quad\quad\quad\quad~~\frac{1}{m^{(\ell)}}\sum_{j=1}^{m^{(\ell)}}\left| \tPsi_s(\zl_j)  \frac{1}{m^{(\ell-1)}}\sum_{i=1}^{m^{(\ell-1)}} \bbw(\zl_j, \zmi_i)\left|\hf_i^{(\ell-1)}(x) - \breve{f}^{(\ell-1)}(\rho,\zmi_i;x) \right|    \right|^{2\beta_{t+1}}\notag\\
&+c_1^{2\beta_t}q_0^{-2\alpha\beta_t}(1-q_1)^{-2\beta_t +1}\times\notag\\
&\quad\quad\quad~\frac{1}{m^{(\ell)}}\sum_{j=1}^{m^{(\ell)}}\left| \tPsi_s(\zl_j)  \frac{1}{m^{(\ell-1)}}\sum_{i=1}^{m^{(\ell-1)}} \left[w(\zl_j, \zmi_i)\breve{f}^{(\ell-1)}(\rho,\zmi_i;x) -  \gl(\rho,\zl_j;x) \right]    \right|^{2\beta_{t+1}}\notag\\
&+  c_0^{2\beta_t}q_1^{-2\beta_t +1}\times\notag\\
&\quad\quad\quad\quad\quad~ \frac{1}{m^{(\ell)}}\sum_{j=1}^{m^{(\ell)}}\left| \tPsi_s(\zl_j)   \frac{1}{m^{(\ell-1)}}\sum_{i=1}^{m^{(\ell-1)}} \bbw(\zl_{j}, \zmi_i)\Big|\hf_i^{(\ell-1)}(x) -  \breve{f}^{(\ell-1)}(\rho,\zmi_i;x)\Big|   \right|^{2\beta_t},\notag
\end{align}
where we simply set $q_1 = \frac{1}{4}$ and  $\overset{a}\leq$ uses Jensen Inequality which is
$$ \left|\frac{1}{m}\sum_{i=1}^m x_i \right|^p \leq  \frac{1}{m}\sum_{i=1}^m \left|x_i\right|^p, ~~ p\geq 1,   $$
and $\bbw(\zl_j, \zmi_i) \geq | w(\zl_j, \zmi_i) |$.

In the following, denote:
\begin{align*}
&\Gamma(t, \ell) = \EE \prod_{i=\ell+1}^L\frac{1}{m^{(i)}}\sum_{\ts\in \cA^{(\ell+1)}}\left|\frac{1}{m^{(\ell)}}\tPsi_{\ts}(\zl_j) \sum^{m^{(\ell)}}_{j=1}\left|\hf_j^{(\ell)}(x) - \breve{f}^{(\ell)}(\rho,\zl_j;x)\right|\right|^{2\beta_t},\\
&\Phi(t, \ell) = \EE \prod_{i=\ell+1}^L \frac{1}{m^{(i)}} \sum_{\ts\in \cA^{(\ell)}} \left| 
\Psi^{(\ell+1)}(\ts)\frac{1}{m^{(\ell-1)}}\sum_{j=1}^{m^{(\ell-1)}}\left[ w(\zl_{\ts_{\ell}},\zmi_{j} )
\breve{f}^{(\ell-1)}(\rho,\zmi_{j};x) -  g^{(\ell)}(\rho,\zl_{\ts_{\ell}};x)\right]     \right|^{2\beta_t},
\end{align*}
and
$$ d_t = c_1^{2\beta_t}q_1^{-2\alpha\beta_t-2\beta_t +1}, \quad e_t=  c_1^{2\beta_t}q_0^{-2\alpha\beta_t}(1-q_1)^{-2\beta_t +1}, \quad  f_t=  c_0^{2\beta_t}q_1^{-2\beta_t +1}.$$

Note that because 
\begin{align}
    &\left\| \frac{1}{m^{(L)}}\sum_{j=1}^{m^{(L)}}u^{(L)}(z_j^{(L)}) \left[\hat{f}^{(L)}_j(x)-\breve{f}(\rho, z^{(L)};x)\right]  \right\|\notag\\
    \leq&   \frac{1}{m^{(L)}}\sum_{j=1}^{m^{(L)}}\left\|u^{(L)}(z_j^{(L)}) \right\| \left|\hat{f}^{(L)}_j(x)-\breve{f}(\rho, z^{(L)};x)\right|\notag\\
    \leq& \frac{1}{m^{(L)}}\sum_{j=1}^{m^{(L)}}\bbu(z_j^{(L)})\left|\hat{f}^{(L)}_j(x)-\breve{f}(\rho, z^{(L)};x)\right|\notag\\
    =& \left|\frac{1}{m^{(L)}}\sum_{j=1}^{m^{(L)}}\bbu(z_j^{(L)})\left|\hat{f}^{(L)}_j(x)-\breve{f}(\rho, z^{(L)};x)\right|\right|.\notag
\end{align}
We have
\begin{align}
    &\E \|\breve{f}(\rho,u;x)-\hf(x) \|^2\label{endd}\\
    =&\E\left\| \frac{1}{m^{(L)}}\sum_{j=1}^{m^{(L)}}u^{(L)}(z_j^{(L)}) \left[\hat{f}^{(L)}_j(x)-\breve{f}(\rho, z^{(L)};x)\right]  \right\|^2\notag\\
    \leq & \E\left|\frac{1}{m^{(L)}}\sum_{j=1}^{m^{(L)}}\bbu(z_j^{(L)})\left|\hat{f}^{(L)}_j(x)-\breve{f}(\rho, z^{(L)};x)\right|\right|^2\notag\\
    =&\Gamma(0, L).\notag
\end{align}
 $\Phi(t,l)$ is bounded in \eqref{l use}, $d_t$, $e_t$, and $f_t$ can be treated as constants when $t\leq L$. Then integrating \eqref{ttend} with $s\in \cA^{(\ell+1)}$, multiplying the both sides by  $\prod_{i=\ell+1}^L\frac{1}{m^{(i)}}$, and taking expectation, for all $\ell\in \{2, \dots, L\}$ and $t\geq 0$, we have
\begin{eqnarray}
\Gamma(t, \ell) \leq d_t  \Gamma(t+1, \ell-1) + e_t  \Phi(t+1, \ell) + f_t \Gamma(t, \ell-1).
\end{eqnarray} 
For all $t\leq L$, we have
$$ d_t \leq d_{L}\vee d_{0}, \quad f_t\leq f_{L}\vee f_{0}.     $$
Let $\gamma = d_{T} \vee f_{T} \vee d_{0} \vee f_{0} \vee 1$,   for all $t\leq L$, we have
\begin{eqnarray}
\Gamma(t, \ell+1) \leq \gamma(\Gamma(t+1, \ell)+ \Gamma(t, \ell)) + \tPhi(t, \ell+1),
\end{eqnarray}
where $ \tPhi(t, \ell) = \Phi(t+1,\ell)e_t$ and $\ell\in [L-1]$.

When $\ell=1$, we have  $\Gamma(t, 1)=0$ for all $t\geq 0$. Then we show that 
\begin{eqnarray}
\Gamma(t, \ell) \leq \sum_{i=1}^{\ell}\gamma^{\ell-i}\sum_{j=0}^{\ell-i}\left(\begin{matrix}
\ell-i\\j
\end{matrix}\right)\tPhi(j+t, i).
\end{eqnarray}
We prove it by induction. When $\ell=1$, the above statement is true.  Suppose at $\ell-1$, the statement is true.  We have
\begin{align}
\Gamma(t, \ell+1)\leq& \sum_{i=1}^{\ell} \gamma^{\ell-i+1} \sum_{j=0}^{\ell-i}\left(\begin{matrix}
\ell-i\\j
\end{matrix}\right)\tPhi(j+t+1,i) +\sum_{i=1}^{\ell} \gamma^{\ell-i+1} \sum_{j=0}^{\ell-i}\left(\begin{matrix}
\ell-i\\j
\end{matrix}\right)\tPhi(j+t,i)+ \tPhi(t, {\ell+1})\notag\\
\overset{a}{=}&\sum_{i=1}^{\ell} \gamma^{\ell-i+1}\left[ \sum_{j=1}^{\ell-i}\left(\begin{matrix}
\ell-i+1\\j
\end{matrix}\right)\tPhi({j+t}, i)+ \tPhi(t,i)+ \tPhi({\ell-i+1+t},i) \right] +\tPhi(t,{\ell+1})\notag\\
=&\sum_{i=1}^{\ell+1}\gamma^{\ell+1-i}\sum_{j=0}^{\ell+1-i}\left(\begin{matrix}
\ell+1-i\\j
\end{matrix}\right)\tPhi(j+t, i), \notag
\end{align} 
where in $\overset{a}=$, we use 
$$ \left(\begin{matrix}
n\\k
\end{matrix}\right) +\left(\begin{matrix}
n\\k+1
\end{matrix}\right) = \left(\begin{matrix}
n+1\\k+1
\end{matrix}\right).$$
In all, we have
\begin{eqnarray}
&&\E\left\| \breve{f}(\rho,u;x)-\hf(x)\right\|^2\notag\\
&\overset{\eqref{endd}}\leq&\Gamma(0, L) \notag\\
& \overset{a}{\leq}&  L\gamma^{L} C^0_{B_T}(c_{M}\vee 1) (e_L\vee e_0) \mathcal{O}\left( \sum_{\ell=1}^{L} \frac{1}{(m^{(j)})^{1+\alpha}} \right)\notag\\
&=&\mathcal{O}\left( \sum_{\ell=1}^{L} \frac{1}{(m^{(j)})^{1+\alpha}} \right).\notag
\end{eqnarray}
where in $\overset{a}=$, we use the fact that for all $\Phi(t+1, \ell)$ has the lowest order $\frac{1}{(m^{(j)})^{1+\alpha}}$  only when $t=0$ and $j=0$, $\frac{1}{(m^{J^(\ell)})^{1+\alpha}} \leq \sum_{\ell=1}^{L} \frac{1}{(m^{(j)})^{1+\alpha}} $,
and  $\gamma$, $C^0_{B_T}$, $e_L$, and $e_0$ only depend on $L, \alpha, c_0, c_1,$ and $c_M$, and can be treated as constants. 


Furthermore, by setting $\alpha = \mathcal{O}(\frac{1}{L})$, we explictly have
\begin{eqnarray}
\E\left\| \breve{f}(\rho,u;x)-\hf(x)\right\|^2\leq \mathcal{O}\left(\sum_{\ell=1}^{L} \frac{L(cc_0\vee c_1^2)^{eL} (c_{M}\vee 1)} {(m^{(\ell)})^{1+\mathcal{O}(\frac{1}{L})}} \right).
\end{eqnarray}




\textbf{Step 4.}  The proof is ended by the fact that
\begin{align}
\E\left\| \hf(x)-  f(\rho,u;x)\right\|^2\leq 2\E\left\| f(\rho,u;x)-\breve{f}(\rho,u;x)\right\|^2 +2\E\left\| \breve{f}(\rho,u;x)-\hf(x)\right\|^2. \nonumber
\end{align}

\end{proof}


 





%\section{Definition}
%We denote $[L] = \{1, 2, \dots, L\}$. Let  $\cSl$ be the set  that consists all ordered pairs in the form of $\{k_1, k_2, \dots, k_{\ell} \}$ with $k_{j}\in [m^{(j)}]$ and $j\in [\ell]$. That is 
%$$ \cS^{(\ell)} = [m^{(1)}] \times [m^{(2)}] \times \cdots \times [m^{\ell}], $$
%where $\times$ is the  Cartesian product. Denote $\zsetl$  be the set that $\{z^{(\ell)}_{j}:~ j\in[m^{(\ell)}]  \} $.   Denote 
%$$  \zSetl=  \{z^{(1)}\}\times \{z^{(1)}\} \times \cdots \times \{z^{(\ell)}\}. $$
 %$\EE[f]$ means taking full expectation on all the random variables. $\EE_{\zsetl}[f]$ (or $\EE_{\zSetl}[f]$) means taking conditional expectation  on $\zsetl$ (or $\zSetl$).


%Consider the discrete NN as:
%$$ \hf^{(0)}(z^{(0)}_j) = z^{(0)}_j, \quad j \in [d],$$
%\begin{eqnarray}
%\hf^{(\ell)}(\zl_j) = \hl\left(\frac{1}{m^{(\ell-1)}}\sum_{i=1}^{m^{(\ell-1)}}  w(\zl_j, \zmi_i)\hf^{(\ell-1)} (\zmi_i) \right), \quad \ell\in [L], ~~j\in [m^{(\ell)}],
%\end{eqnarray}
%and 
%\begin{eqnarray}
%\hf^{o} = \frac{1}{m^{(L)}}\sum_{i=1}^{m^{(L)}}\hf^{(L)}(\zL_i) u(\zL_i).
%\end{eqnarray}



%We consider the continuous NN as:
%$$f^{(0)}(z^{(0)}_j) = z^{(0)}_j, \quad j \in [d],  $$
%\begin{eqnarray}\label{def g}
%g^{(\ell)}(\zl) = \E_{\zmi} f^{(\ell-1)}(\zmi) w(\zl, \zmi), \quad \ell\in [L], ~~j\in [m^{(\ell)}],
%\end{eqnarray}
%\begin{eqnarray}\label{def f}
%f^{(\ell)}(\zl) = \hl\left(g^{(\ell)}(\zl)\right),
%\end{eqnarray}
%and 
%\begin{eqnarray}
%f^{o} = \E_{\zL} f^{(L)}(\zL) u(\zL).
%\end{eqnarray}
%Thus our destination is to bound 
%\begin{eqnarray}
%\E | \hf^{o} - f^{o} |^2
%\end{eqnarray}
%We then introduce  the following functions:
%\begin{eqnarray}\label{def bf}
%\bf^{(\ell)}(\zl_j) = \hl ( \gl(\zl_j) ) +\nabla \hl( \gl(\zl_j) )\left[ \frac{1}{m^{(\ell-1)}} \sum_{i=1}^{m^{(\ell-1)}} w(\zl_j, \zmi_i)\bf^{(\ell-1)}(\zmi_i)- \gl(\zl_j) \right],
%\end{eqnarray}
%where $\ell\in [L]$ and $j\in [m^{(\ell)}]$. And
%\begin{eqnarray}\label{ffo}
%\bf^{o} = \frac{1}{m^{(L)}}\sum_{i=1}^{m^{(L)}}\bf^{(L)}(\zL_i)u(\zL_i).
%\end{eqnarray}

%In the same way, we define $\Jl(z^{(1)}, \dots, z^{(\ell)})$. Let
%$$J^{(1)}(z^{(1)}_j) = h\left( \frac{1}{d}\sum_{i=1}^d w(z^{(1)}_j, z^{0}_i), z^{(0)}_i\right), $$
%$$
%\Jl(z^{(1)}, \dots, z^{(\ell)})=\hl ( \gl(\zl) ) +\nabla \hl( \gl(\zl) )\left[ w(\zl, \zmi)J^{(\ell-1)}(\zmi)- \gl(\zl) \right],
%$$
%where $\ell\in[2, 3,\dots, L]$,
%and 
%$$\tJ(z^{(1)}, \dots, z^{(L)}) = J^{(L)}(z^{(1)}, \dots, z^{(L)})u( z^{(L)}) - f^{o}.$$
%e will show that $\E\tJ(z^{(1)}, \dots, z^{(L)})=0 $.





%\section{Proof of Theorem \ref{var}}
%\begin{enumerate}[Step 1.]
%\item\label{step 1} We prove 
%\begin{equation}\label{stt1}
% \E_{\zSetlm}\bf^{(\ell)}(\zl_j) = f^{(\ell)}(\zl_j), ~~\ell\in [L],
%\end{equation} 
%and 
%$$ \E_{\{z\}_{\cS^{L}}}\bf^{o} = f^o. $$
%\begin{proof}
%We prove it by induction. When $\ell=1$, the statement is true. Suppose at $\ell-1$, the statement is true.  We consider $\ell$. For all $j\in m^{(\ell)}$, we have
%\begin{eqnarray}
%&&\EE_{\zSetlm}\bf^{(\ell)}(\zl_j)\notag\\
% &=& \EE_{\{\zmi\}}\left[\EE_{\{z\}_{\cS^{\ell-2}}}\bf^{(\ell)}(\zl_j)\right]\notag\\
% &\overset{\eqref{def bf}}{=}&  \EE_{\{\zmi\}}\left[\hl ( \gl(\zl_j) )\right]\notag\\
% &&\!\!\!\!\!\!\! +\EE_{\{\zmi\}}\left\{\nabla \hl( \gl(\zl_j) )\left[ \frac{1}{m^{(\ell-1)}} \sum_{i=1}^{m^{(\ell-1)}} w(\zl_j, \zmi_i)\EE_{\{z\}_{\cS^{\ell-2}}}\left[\bf^{(\ell-1)}(\zmi_i)\right]- \gl(\zl_j) \right]\right\}\notag\\
%&\overset{a}=&\!\!\!\!\!\!\! \hl ( \gl(\zl_j) ) +\EE_{\{\zmi\}}\nabla \hl( \gl(\zl_j) )\left[ \frac{1}{m^{(\ell-1)}} \sum_{i=1}^{m^{(\ell-1)}} w(\zl_j, \zmi_i)f^{(\ell-1)}(\zmi_i)- \gl(\zl_j) \right]\notag\\
% &\overset{\eqref{def g}}{=}&\hl ( \gl(\zl_j) ) \notag\\
% &\overset{\eqref{def f}}{=}& f^{(\ell)}(\zl_j),\notag
%\end{eqnarray}
%where  $\overset{a}=$ applies \eqref{stt1} on %$\ell-1$.
%Then 
%\begin{eqnarray}
%\E \bf^o = \E_{\{z\}^L} \frac{1}{m^{(L)}}\sum_{j=1}^{m^{(L)}}f^{(L)}(z_j^{(L)}) u_j^{(L)} = f^{o}.
%\end{eqnarray}

%\end{proof}

%\item  We compute 
%$$\E| \bf^{o}-f^{o}|^2,    $$
%\begin{proof}
%We first show that
% \begin{eqnarray}\label{bff1}
% \bf^{o} =  \prod_{\ell=1}^L \frac{1}{m^{(\ell)}}\left(\sum_{s\in \cS^{(L)}} J^{L}(z^{(1)}_{s_1}, \dots,z^{(1)}_{s_L}) u(z^{(L)}_{s_L})\right).
% \end{eqnarray}

%Clearly, we have $\bf^{(1)} (z^{(1)}_j) =J^{(1)} (z^{(1)}_j) =f^{(1)} (z^{(1)}_j)$, for all $j\in [m^{(1)}]$.  Then we can  verify that  for all  $j\in  [m^{(2)}]$, 
%\begin{eqnarray}\label{ffo0}
%\bf^{2}(z^{(2)}_{j}) = \frac{1}{m^{(1)}} \sum_{i=1}^{m^{(1)}}J^{2}(z^{(1)}_{i}, z^{(2)}_{j}).
%\end{eqnarray}


%We then prove for all $\ell \in \{ 3, \dots, L\}$ and  $j\in [ m^{(\ell)}]$, we have 
%\begin{eqnarray}\label{ffo1}
%\bf^{\ell}(z^{(\ell)}_{j}) =  \prod_{k=1}^{\ell-1} \frac{1}{m^{(k)}}\left( \sum_{s\in\cS^{(\ell-1)}}J^{\ell}(z^{(1)}_{s_1}, \dots,z^{(\ell-1)}_{s_{\ell-1}}, z^{(\ell)}_{j})\right). 
%\end{eqnarray}
%Suppose the above statement is  true at $\ell-1$, then from \eqref{def bf}, we have
%\begin{eqnarray}
%&&\bf^{(\ell)}(\zl_{j})\notag\\
% &\overset{\eqref{def bf}}=& \hl ( \gl(\zl_j) ) -\nabla \hl( \gl(\zl_j) ) \gl(\zl_j)\notag\\
% &&+ \nabla \hl( \gl(\zl_j) ) \frac{1}{m^{(\ell-1)}} \sum_{i=1}^{m^{(\ell-1)}} w(\zl_j, \zmi_i)\bf^{(\ell-1)}(\zmi_i)\notag\\
% &\overset{a}=&\hl ( \gl(\zl_j) ) -\nabla \hl( \gl(\zl_j) ) \gl(\zl_j) \notag\\
% &&\!\!\!\!\!\!\!\!\!\!\!\!\!\!\!+ \nabla \hl( \gl(\zl_j) ) \frac{1}{m^{(\ell-1)}} \sum_{i=1}^{m^{(\ell-1)}}\left[\prod_{k=1}^{\ell-2} \frac{1}{m^{(k)}}\left(\sum_{s\in\cS^{\ell-2}} J^{(\ell-1)}(z^{(1)}_{s_1}, \dots,z^{(\ell-2)}_{s_{\ell-2}}, z^{(\ell-1)}_i)\right)w(\zl_{j}, \zmi_{i})\right]\notag\\
%&=& \hl ( \gl(\zl_j) ) -\nabla \hl( \gl(\zl_j) ) \gl(\zl_j) \notag\\
% &&+\nabla \hl( \gl(\zl_j) )  \prod_{k=1}^{\ell-1} \frac{1}{m^{(k)}}\left(\sum_{s\in\cS^{\ell-1}} J^{(\ell-1)}(z^{(1)}_{s_1}, \dots,z^{(\ell-1)}_{s_{\ell-1}})w(\zl_{j}, \zmi_{s_{\ell-1}})\right)\notag\\
% &=&  \prod_{k=1}^{\ell-1} \frac{1}{m^{(k)}}\left[\sum_{s\in\cS^{\ell-1}} \left(\hl ( \gl(\zl_j) ) -\nabla \hl( \gl(\zl_j) ) \gl(\zl_j)\right)\right] \notag\\
% &&+ \nabla \hl( \gl(\zl_j) )\prod_{k=1}^{\ell-1} \frac{1}{m^{(k)}}\left(\sum_{s\in\cS^{\ell-1}} J^{(\ell-1)}(z^{(1)}_{s_1}, \dots,z^{(\ell-1)}_{s_{\ell-1}})w(\zl_{j}, \zmi_{s_{\ell-1}})\right)\notag\\
% &=&\prod_{k=1}^{\ell-1} \frac{1}{m^{(k)}}\left( \sum_{s\in\cS^{(\ell-1)}}J^{(\ell)}(z^{(1)}_{s_1}, \dots,z^{(\ell-1)}_{s_{\ell-1}}, z^{(\ell)}_{j})\right),\notag
%\end{eqnarray}
%where in $\overset{a}=$, we use \eqref{ffo1} on $\ell-1$. So we obtain \eqref{ffo1}  on $\ell$.  Then plugging \eqref{ffo1} with $\ell =L$ into \eqref{ffo}, we can obtain \eqref{bff1}. Also by the same technique of Step \ref{step 1}, we can obtain 
%\begin{eqnarray}\label{exp z}
%\EE_{z^{(1)}, \dots, z^{(\ell-1)}} J^{(\ell)}(z^{(1)}, \dots, z^{(\ell)}) = f^{(\ell)}(z^{(\ell)}), ~~\ell\in [L],
%\end{eqnarray}
%and
%\begin{eqnarray}{exp l}
%\EE_{z^{(1)}, \dots, z^{(L)}} J^{(L)}(z^{(1)}, \dots, z^{(L)})u( z^{(L)})  = f^{o}.
%\end{eqnarray}
%Recall
%$$\tJ(z^{(1)}, \dots, z^{(L)}) = J^{(L)}(z^{(1)}, \dots, z^{(L)})u( z^{(L)}) - f^{o},$$
%  $\E_{z^{(1)}, \dots, z^{(L)}}\tJ(z^{(1)}, \dots, z^{(L)}) = 0. $. Now we are ready to bound $\E|\bf^{o} - f^o|$.
%\begin{eqnarray}\label{lin}
%&&\E | \bf^{o} - f^o |^2\\
%&=&\prod_{\ell=1}^{L}\frac{1}{(m^{(\ell)})^2}\E\left| \sum_{s\in \cS^{(L)}} \tJ(z^{(1)}_{s_1}, \dots, z^{(L)}_{s_L})     \right|^2\notag\\
%&=&\prod_{\ell=1}^{L}\frac{1}{(m^{(\ell)})^2}\E \left[ \sum_{s^a\in \cS^{(L)}}\sum_{s^b\in \cS^{(L)}} \tJ(z^{(1)}_{s^a_1}, \dots, z^{(L)}_{s^a_L}) \tJ(z^{(1)}_{s^b_1}, \dots, z^{(L)}_{s^b_L})      \right]\notag\\
%&=&\sum_{s^a\in \cS^{(L)}}\sum_{s^b\in \cS^{(L)}}\left[ \prod_{\ell=1}^{L}\frac{1}{(m^{(\ell)})^2} \E_{z^{(1)}_{s^a_1}, \dots, z^{(L)}_{s^a_L}}\E_{z^{(1)}_{s^b_1}, \dots, z^{(L)}_{s^b_L}}\tJ(z^{(1)}_{s^a_1}, \dots, z^{(L)}_{s^a_L}) \tJ(z^{(1)}_{s^b_1}, \dots, z^{L}_{s^b_L}) \right]\notag\\
%&\overset{a}{=}&\sum_{s^a\in \cS^{(L)}}\sum_{s^b\in \cS^{(L)}}\left[ \prod_{\ell=1}^{L}\frac{1}{(m^{(\ell)})^2} \E_{\zl_{s^a_\ell}, \ell\in p^{ab}}\E_{\zl_{s^a_\ell}, \ell\in q^{ab}}\E_{\zl_{s^b_\ell}, \ell\in q^{ab}}\tJ(z^{(1)}_{s^a_1}, \dots, z^{(L)}_{s^a_L}) \tJ(z^{(1)}_{s^b_1}, \dots, z^{L}_{s^b_L}) \right]\notag\\
%&\overset{b}{=}&\sum_{s^a\in \cS^{(L)}}\sum_{s^b\in \cS^{(L)}}\left[ \prod_{\ell=1}^{L}\frac{1}{(m^{(\ell)})^2} \E_{\zl_{s^a_\ell}, \ell\in p^{ab}}\left|\E_{\zl_{s^a_\ell}, \ell\in q^{ab}}\tJ(z^{(1)}_{s^a_1}, \dots, z^{(L)}_{s^a_L})\right|^2  \right]\notag\\
%&\overset{c}{=}&\sum_{\ell=0}^L \sum_{\mathcal{a}\in \mathcal{C}^\ell}\left[ \left(\prod_{k\in \mathcal{a}}\frac{1}{m^{(k)}} \prod_{k\in \mathcal{a}^c}\frac{m^{(k)}-1}{m^{(k)}}\right) \E_{z^{(i)}, i\in \mathcal{a}}\left|\E_{ z^{(j)}, j\in \mathcal{a}^c}\tJ(z^{(1)}, \dots, z^{(L)})\right|^2  \right]\notag\\
%&\overset{d}{=}&\sum_{\ell=1}^L \sum_{\mathcal{a}\in \mathcal{C}^\ell}\left[ \left(\prod_{k\in \mathcal{a}}\frac{1}{m^{(k)}} \prod_{k\in \mathcal{a}^c}\frac{m^{(k)}-1}{m^{(k)}}\right) \E_{z^{(i)}, i\in \mathcal{a}}\left|\E_{ z^{(j)}, j\in \mathcal{a}^c}\tJ(z^{(1)}, \dots, z^{(L)})\right|^2  \right].\notag
%\end{eqnarray}
%We  explain \eqref{lin}.  In $\overset{a}=$, we denote $p^{ab} = \{\ell: s^a_\ell = s^b_\ell, ~ \ell \in [L]\}$ and $q^{ab} = \{\ell: s^a_\ell \neq s^b_\ell, \ell \in [L]\}$. In $\overset{b}=$,  given $\zl_{s^a_\ell}$ with $\ell\in p^{ab}$, $\tJ(z^{(1)}_{s^a_1}, \dots, z^{(L)}_{s^a_L})$ and $\tJ(z^{(1)}_{s^b_1}, \dots, z^{L}_{s^b_L})$ are independent, so 
%\begin{eqnarray}
%&&\E_{\zl_{s^a_\ell}, \ell\in q^{ab}}\E_{\zl_{s^b_\ell}, \ell\in q^{ab}}\tJ(z^{(1)}_{s^a_1}, \dots, z^{(L)}_{s^a_L}) \tJ(z^{(1)}_{s^b_1}, \dots, z^{L}_{s^b_L})\notag\\
%& =& \E_{\zl_{s^a_\ell}, \ell\in q^{ab}}\tJ(z^{(1)}_{s^a_1}, \dots, z^{(L)}_{s^a_L})\E_{\zl_{s^b_\ell}, \ell\in q^{ab}} \tJ(z^{(1)}_{s^b_1}, \dots, z^{L}_{s^b_L}) \notag\\
%&=&    \left|\E_{\zl_{s^a_\ell}, \ell\in q^{ab}} \tJ(z^{(1)}_{s^a_1}, \dots, z^{(L)}_{s^a_L})\right|^2.
%\end{eqnarray}
%In $\overset{c}=$, we denote $\mathcal{C}^\ell$ as the set of all the $\ell$-combinations of $[L]$, specially $\mathcal{C}^0 = \{\varnothing\}$. Then for all $\mathcal{a}\in \mathcal{A}$, we denote $\mathcal{a}^c = [L] -\mathcal{a}$.  Then for each $\ell\in [m] $, consider  we sample $2$ numbers from $m^{(\ell)}$ with replacement, There are $m^{(\ell)}$ possibilities if the two numbers are the same and  $m^{(\ell)}m^{(\ell)-1}$ possibilities  if the two numbers are different. In $\overset{d}{=}$, we use when $\ell = 0$,  
%$$ \E_{ z^{(j)}, j\in \mathcal{a}^c}\tJ(z^{(1)}, \dots, z^{(L)}) = \E_{ z^{(1)}, \dots, z^{(L)}}\tJ(z^{(1)}, \dots, z^{(L)}) = 0. $$
%\end{proof} 

%\item Then the remaining to do is to bound
%$$\E| \bf^{o}-\hf^{o}|^2,    $$
%which is carried out in this step.  
%\begin{proof}
%Denote  
%$$ \cA^{(\ell)} = [m^{(\ell)}] \times [m^{(\ell+1)}] \times \cdots \times [m^{(L)}].
% $$
% Let 
% $$\Psi^{(L+1)}(\ts) = u(z^{(L)}_{\ts_L}), ~~ \ts\in \cA^{(L)},$$
% and for $\ell \in \{2, \cdots, L \}$ and  $\ts\in \cA^{(\ell-1)}$,  we define
% $$ \Psi^{(\ell)}(\ts) = u(z^{(L)}_{\ts_L})  \left(\prod_{i = \ell}^{L} w(z^{(i)}_{\ts_i}, z^{(i-1)}_{\ts_{i-1}})\right), $$
%For for $\ell\in \{2, 3, \dots, L\}$, and $t\geq0$,  by setting $\beta_t= (1+\alpha)^{t+1}\geq 1$, we first consider bounding
%\begin{eqnarray}\label{l use}
%\EE\sum_{\ts\in \cA^{(\ell)}}  \left(\prod_{i=\ell}^L \frac{1}{m^{(i)}}\right) \left| 
%\Psi^{(\ell+1)}(\ts)\frac{1}{m^{(\ell-1)}}\sum_{j=1}^{m^{(\ell-1)}}\left[ w(\zl_{\ts_{\ell}},\zmi_{j} )
%\bf^{(\ell-1)}(\zmi_{j}) -  g^{(\ell)}(\zl_{\ts_{\ell}})\right]     \right|^{2\beta_t}.
%\end{eqnarray}


%When $\ell=1$, \eqref{l use} equals to $0$.  When $\ell\geq 2$, from  \eqref{ffo0} and \eqref{ffo1}, we have
%\begin{eqnarray}
%&&\EE\sum_{\ts\in \cA^{(\ell)}}  \left(\prod_{i=\ell}^L \frac{1}{m^{(i)}}\right) \left| 
%\Psi^{(\ell+1)}(\ts)\frac{1}{m^{(\ell-1)}}\sum_{j=1}^{m^{(\ell-1)}}\left[ w(\zl_{\ts_{\ell}},\zmi_{j} )
%\bf^{(\ell-1)}(\zmi_{j}) -  g^{(\ell)}(\zl_{\ts_{\ell}})\right]     \right|^{2\beta_t}\notag\\
%&=&
%\prod_{i=\ell}^L \frac{1}{m^{(i)}}\EE\sum_{\ts\in \cA^{(\ell)}} \notag\\
%&&
%\left|  \prod^{\ell-1}_{j=1}\frac{1}{(m^{(j)})}\Psi^{(\ell+1)}(\ts)\sum_{\hs\in \cS^{\ell-2}}\sum_{j=1}^{m^{(\ell-1)}}\left(w(z^{(\ell)}_{\ts_{\ell}}, z^{(\ell-1)}_j)J^{\ell-1}(z^{(1)}_{\hs_1}, \dots, z^{(\ell-2)}_{\hs_\ell-2}, \zmi_{j}) - g^{(\ell)}(\zl_{\ts_{\ell}})\right) \right|^{2\beta_t}\notag\\
%&\overset{a}=&
%\prod^{\ell-1}_{j=1}\frac{1}{(m^{(j)})^{2\beta_t}} 
%\EE_{z^{(\ell)}, \dots, z^{(L)}} \cdot\notag\\
%&&\E_{\{z\}_{\cS^{\ell-1}}}\left|  \left[u(z^{(L)}) \prod_{i = \ell+1}^{L} w(z^{(i)}, z^{(i-1)})\sum_{\hs\in \cS^{\ell-1}}\left(w(z^{(\ell)}_{\ts_{\ell}}, z^{(\ell-1)}_{\hs_{\ell-1}})J^{\ell-1}(z^{(1)}_{\hs_1}, \dots, z^{(\ell-1)}_{\hs_{\ell-1}}) - g^{(\ell)}(\zl)\right)\right] \right|^{2\beta_t}\notag\\
%&\overset{b}{=}&\prod^{\ell-1}_{j=1}\frac{1}{(m^{(j)})^{2\beta_t}}\EE_{z^{(\ell)}, \dots, z^{(L)}} \E_{\{z\}_{\cS^{\ell-1}}}\left|\sum_{\hs\in \cS^{(\ell-1)}}  \left[\bar{J}^{\ell}(z^{(1)}_{\hs_1}, \dots, z^{(\ell-1)}_{\hs_{\ell-1}})\right] \right|^{2\beta_t}\notag\\
%&\overset{c}{=}&\prod^{\ell-1}_{j=1}\frac{1}{(m^{(j)})^{2\beta_t}} \EE_{z^{(\ell)}, \dots, z^{(L)}} C^1_{\beta_t}\left[ \left(\prod^{\ell-1}_{j=1}m^{(j)}\right)\E_{z^{(1)}, \dots, z^{(\ell-1)}}\left| \bar{J}^{\ell}(z^{(1)}, \dots, z^{(\ell-1)}) \right|^{2\beta_t}  \right]\notag\\
%&&+ \prod^{L}_{j=1}\frac{1}{(m^{(j)})^{2\beta_t}}\EE_{z^{(\ell)}, \dots, z^{(L)}} C^2_{\beta_t}\left( \left(\prod^{\ell-1}_{j=1}m^{(j)}\right)\E_{z^{(1)}, \dots, z^{(\ell-1)}}\left| \bar{J}^{\ell}(z^{(1)}, \dots, z^{(\ell-1)}) \right|^2  \right)^{\beta_t}\notag\\
%&\overset{c}{\leq}&  C^0_{\beta_t}\prod^{L}_{j=1}\frac{1}{(m^{(j)})^{\beta_t}}\E_{z^{(1)}, \dots, z^{(L)}}|\bar{J}^{\ell}(z^{(1)}, \dots, z^{\ell-1)})|^{2\beta_t}\notag\\
%&\overset{d}{\leq}& C^0_{\beta_t} (c_{M_2}\vee 1)\prod^{\ell-1}_{j=1}\frac{1}{(m^{(j)})^{\beta_t}}.
%\end{eqnarray}
%We explain \eqref{l use}. In $\overset{a}=$, we take expectation on $\{z\}_{\cA^\ell}$. In $\overset{b}=$, we denote
%$$ \bar{J}^{\ell}(z^{(1)}_{\hs_1}, \dots, z^{(\ell-1)}_{_{\hs_{\ell-1}}}) =  u(z^{(L)}) \prod_{i = \ell+1}^{L} w(z^{(i)}, z^{(i-1)})\left(w(z^{(\ell)}, z^{(\ell-1)}_{\hs_{\ell-1}})J^{\ell-1}(z^{(1)}_{\hs_1}, \dots, z^{(\ell-1)}_{\hs_{\ell-1}}) - g^{(\ell)}(\zl)\right). $$
%$\overset{c}=$ is because that all $\bar{J}^{\ell}(z^{(1)}_{s_1}, \dots, z^{(L)}_{s_L})$ are independent  given $\{z^{(\ell)}, \dots, z^{(L)}\}$ and is obtained by Rosenthal Inequality (Refer to Lemma \ref{rosenthal}).  In $\overset{d}=$, we use Jensen inequality,   given $\{z^{(\ell)}, \dots, z^{(L)}\}$,  we have
%$$  \left(\E_{z^{(1)}, \dots, z^{\ell-1}}\left| \bar{J}^{\ell}(z^{(1)}, \dots, z^{(\ell-1)})   \right|^2\right)^{\beta_t} \leq  \E_{z^{(1)}, \dots, z^{\ell-1}}\left| \bar{J}^{\ell}(z^{(1)}, \dots, z^{(\ell-1)} \right|^{2\beta_t} $$ 
%and 
%$$  \prod^{\ell-1}_{j=1}\frac{1}{(m^{(j)})^{2\beta_t-1}} \leq \prod^{\ell-1}_{j=1}\frac{1}{(m^{(j)})^{\beta_t}} $$
%since $\beta\geq1$. $\overset{e}\leq$ uses Assumption %\ref{ass:3}.

%On the other hand,  for any $\ell\in \{2, \dots, L\}$ and $j\in [m^{\ell}]$, from Lemma \ref{lip}, we have
%\begin{eqnarray}\label{tmt}
%&&\!\!\!\!\!\!\!\!\!\!\left|\hf^{(l)}(\zl_j)  -  \hl(\gl(\zl_j)) - \left[\nabla  \hl(\gl(\zl_j))\right]\left[  \frac{1}{m^{(\ell-1)}}\sum_{i=1}^{m^{(\ell-1)}} w(\zl_j, \zmi_i)\hf^{(\ell-1)}(\zmi_i) -  \gl(\zl_j) \right]    \right|\notag\\
%&\leq& c\left| \frac{1}{m^{(\ell-1)}}\sum_{i=1}^{m^{(\ell-1)}} w(\zl_j, \zmi_i)\hf^{(\ell-1)}(\zmi_i) -  \gl(\zl_j)     \right|^{1+\alpha}. 
%\end{eqnarray}
%Denote $\tPsi_s(z^{(\ell)}) = \Psi^{(\ell+2)}(\ts)w(z^{\ell+1}_{s_{\ell+1}}, \zl)$ where $\ell \in \{2, \dots, L-1 \}$ and $s\in \cA^{(\ell+1)}$. Then
%\begin{eqnarray}\label{onet}
%&&\left|\frac{1}{m^{(\ell)}} \sum^{m^{(\ell)}}_{j=1}\tPsi_s(\zl_j)\left(\hf^{(\ell)}(\zl_j) - \bf^{(\ell)}(\zl_j)\right)\right|\notag\\
%&\leq&\frac{1}{m^{(\ell)}}\sum^{m^{(\ell)}}_{j=1}\left|\tPsi_s(\zl_j)\right|\left| \hf^{(\ell)}(\zl_j) - \bf^{(\ell)}(\zl_j)\right|\notag\\
%&\leq& \frac{1}{m^{(\ell)}}\sum^{m^{(\ell)}}_{j=1}\left|\tPsi_s(\zl_j)\right|\dot\notag\\
%&&\!\!\!\!\!\!\!\!\!\!\left|\hf^{(\ell)}(\zl_j)  -  \hl(\gl(\zl_j)) - \left[\nabla  \hl(\gl(\zl_j))\right]\left[  \frac{1}{m^{(\ell-1)}}\sum_{i=1}^{m^{(\ell-1)}} w(\zl_j, \zmi_i)\hf^{(\ell-1)}(\zmi_i) -  \gl(\zl_j) \right]    \right|\notag\\
%&&+ \frac{1}{m^{(\ell)}}\sum^{m^{(\ell)}}_{j=1}\left|\tPsi_s(\zl_j)\right|\dot\notag\\
%&&\!\!\!\!\!\!\!\!\!\!\left|\bf^{(\ell)}(\zl_j)  -  \hl(\gl(\zl_j)) - \left[\nabla  \hl(\gl(\zl_j))\right]\left[  \frac{1}{m}\sum_{i=1}^m w(\zl_j, \zmi_i)\hf^{(\ell-1)}(\zmi_i) -  \gl(\zl_j) \right]    \right|\notag\\
%&\overset{a}{\leq}&\frac{c}{m^{(\ell)}}\sum^{m^{(\ell)}}_{j=1}\left|\tPsi_s(\zl_j)\right|\left| \frac{1}{m^{(\ell-1)}}\sum_{i=1}^{m^{(\ell-1)}} w(\zl_j, \zmi_i)\hf^{(\ell-1)}(\zmi_i) -  \gl(\zl_j)     \right|^{1+\alpha}\notag\\
%&&+\frac{1}{m^{\ell}}\sum^{m^{(\ell)}}_{j=1}\left|\tPsi_s(\zl_j)\right|\left| \left[\nabla  \hl(\gl(\zl_j))\right]\left[  \frac{1}{m}\sum_{i=1}^m w(\zl_j, \zmi_i)\left(\hf^{(\ell)}(\zmi_i) -  \bf^{(\ell-1)}(\zmi_i)\right) \right]  \right|\notag\\
%&\overset{b}{\leq}&\frac{c}{m^{(\ell)}}\left|\tPsi_s(\zl_j) \frac{1}{m^{(\ell-1)}}\sum_{i=1}^{m^{(\ell-1)}}\left[ w(\zl_j, \zmi_i)\hf^{(\ell-1)}(\zmi_i) -  \gl(\zl_j) \right]    \right|^{1+\alpha}\notag\\
%&&+\frac{c_0}{m^{(\ell)}}\sum^{m^{(\ell)}}_{j=1}\left|\tPsi_s(\zl_j)\right|\left| \left[  \frac{1}{m^{(\ell-1)}}\sum_{i=1}^{m^{(\ell-1)}} w(\zl_j, \zmi_i)\left(\hf^{(\ell)}(\zmi_i) -  \bf^{(\ell-1)}(\zmi_i)\right) \right]  \right|, \notag
%\end{eqnarray}
%where  $\overset{a}\leq$ uses \eqref{tmt} and  $\overset{b}\leq$ uses Assumption \ref{ass:2}.
%Furthermore, for the second term on the right hand side of \eqref{onet},  we have
%\begin{eqnarray}
%&&\left|\tPsi_s(\zl_j) \frac{1}{m^{(\ell-1)}}\sum_{i=1}^{m^{(\ell-1)}} \left[w(\zl_j, \zmi_i)\hf^{(\ell-1)}(\zmi_i) -  \gl(\zl_j) \right]    \right|\notag\\
%&\leq&  \left| \tPsi_s(\zl_j)  \frac{1}{m^{(\ell-1)}}\sum_{i=1}^{m^{(\ell-1)}} w(\zl_j, \zmi_i)\left(\hf^{(\ell-1)}(\zmi_i) - \bf^{(\ell-1)}(\zmi_i) \right)    \right|\notag\\
%&&+\left| \tPsi_s(\zl_j) \frac{1}{m^{(\ell-1)}}\sum_{i=1}^{m^{(\ell-1)}} \left[w(\zl_j, \zmi_i)\bf^{(\ell-1)}(\zmi_i) -  \gl(\zl_j)   \right] \right|.\notag
%\end{eqnarray}
%From Lemma \ref{jcon}, we have
%\begin{eqnarray}\label{onea}
%&&\left|\tPsi_s(\zl_j)  \frac{1}{m^{(\ell-1)}}\sum_{i=1}^{m^{(\ell-1)}} \left[w(\zl_j, \zmi_i)\hf^{(\ell-1)}(\zmi_i) -  \gl(\zl_j) \right]    \right|^{1+\alpha}\\
%&\leq&  (1-q_0)^{-\alpha}\left| \tPsi_s(\zl_j) \frac{1}{m^{(\ell-1)}}\sum_{i=1}^{m^{(\ell-1)}}\left[ w(\zl_j, \zmi_i)\left(\hf^{(\ell-1)}(\zmi_i) - \bf^{(\ell-1)}(\zmi_i) \right) \right]   \right|^{1+\alpha}\notag\\
%&&+q_0^{-\alpha}\left| \tPsi_s(\zl_j)  \frac{1}{m^{(\ell-1)}}\sum_{i=1}^{m^{(\ell-1)}}  w(\zl_j, \zmi_i)\bf^{(\ell-1)}(\zmi_i) -  \gl(\zl_j)     \right|^{1+\alpha},\notag
%\end{eqnarray}
%where we simply set  $q_0 = \frac{3}{4}$. 

%Plugging \eqref{onea} into \eqref{onet}, we have for for all $\ell\in \{2, \dots, L-1\}$ and $s\in \cA^{\ell+1}$, 
%\begin{eqnarray}
%&&\left|\frac{1}{m^{(\ell)}} \sum^{m^{(\ell)}}_{j=1}\tPsi_s(\zl_j)\left[\hf^{(\ell)}(\zl_j) - \bf^{(\ell)}(\zl_j)\right]\right|\\
%&\leq&c(1-q_0)^{-\alpha}\frac{1}{m^{(\ell)}}\sum_{j=1}^{m^{(\ell)}}\left| \tPsi_s(\zl_j)  \frac{1}{m^{(\ell-1)}}\sum_{i=1}^{m^{(\ell-1)}} w(\zl_j, \zmi_i)\left(\hf^{(\ell-1)}(\zmi_i) - \bf^{(\ell-1)}(\zmi_i) \right)    \right|^{1+\alpha}\notag\\
%&&+c q_0^{-\alpha}\frac{1}{m^{(\ell)}}\sum_{j=1}^{m^{(\ell)}}\left| \tPsi_s(\zl_j)  \frac{1}{m^{(\ell-1)}}\sum_{i=1}^{m^{(\ell-1)}} \left[w(\zl_j, \zmi_i)\bf^{(\ell-1)}(\zmi_i) -  \gl(\zl_j)\right]     \right|^{1+\alpha}\notag\\
%&&+ \frac{c_0}{m^{(\ell)}}\sum_{j=1}^{m^{(\ell)}}\left|\tPsi_s(\zl_j)   \frac{1}{m^{(\ell-1)}}\sum_{i=1}^{m^{(\ell-1)}} w(\zl_{j}, \zmi_i)\left(\hf^{(\ell)}(\zmi_i) -  \bf^{(\ell-1)}(\zmi_i)\right)   \right|.\notag
%\end{eqnarray}
%Finally using  Lemma \ref{jcon} again, for all $\ell\in \{2, \dots, L-1\}$ and $s\in \cA^{\ell+1}$,  we obtain
%\begin{eqnarray}\label{ttend}
%&&\left|\frac{1}{m^{(\ell)}} \sum^{m^{(\ell)}}_{j=1}\tPsi_s(\zl_j)\left[\hf^{(\ell)}(\zl_j) - \bf^{(\ell)}(\zl_j)\right]\right|^{2\beta_t}\\
%&\leq&c^{2\beta_t}q_1^{-2\alpha\beta_t-2\beta_t +1}\cdot\notag\\
%&&\left(\frac{1}{m^{(\ell)}}\sum_{j=1}^{m^{(\ell)}}\left| \tPsi_s(\zl_j)  \frac{1}{m^{(\ell-1)}}\sum_{i=1}^{m^{(\ell-1)}} w(\zl_j, \zmi_i)\left(\hf^{(\ell-1)}(\zmi_i) - \bf^{(\ell-1)}(\zmi_i) \right)    \right|^{1+\alpha}\right)^{2\beta_t}\notag\\
%&&+c^{2\beta_t}q_0^{-2\alpha\beta_t}(1-q_1)^{-2\beta_t +1}\cdot\notag\\
%&&\left(\frac{1}{m^{(\ell)}}\sum_{j=1}^{m^{(\ell)}}\left| \tPsi_s(\zl_j)  \frac{1}{m^{(\ell-1)}}\sum_{i=1}^{m^{(\ell-1)}} w(\zl_j, \zmi_i)\bf^{(\ell-1)}(\zmi_i) -  \gl(\zl_j)     \right|^{1+\alpha}\right)^{2\beta_t}\notag\\
%&&+ c_0^{2\beta_t}q_1^{-2\beta_t +1}\cdot\notag\\
%&&\left(\frac{1}{m^{(\ell)}}\sum_{j=1}^{m^{(\ell)}}\left|\tPsi_s(\zl_j) \left[  \frac{1}{m}\sum_{i=1}^m w(\zl_{j}, \zmi_i)\left(\hf^{(\ell)}(\zmi_i) -  \bf^{(\ell-1)}(\zmi_i)\right) \right]  \right|\right)^{2\beta_t},\notag\\
%&\overset{a}{\leq}&c^{2\beta_t}q_1^{-2\alpha\beta_t-2\beta_t +1}\cdot\notag\\
%&&\frac{1}{m^{(\ell)}}\sum_{j=1}^{m^{(\ell)}}\left| \tPsi_s(\zl_j)  \frac{1}{m^{(\ell-1)}}\sum_{i=1}^{m^{(\ell-1)}} w(\zl_j, \zmi_i)\left(\hf^{(\ell-1)}(\zmi_i) - \bf^{(\ell-1)}(\zmi_i) \right)    \right|^{2\beta_{t+1}}\notag\\
%&&+c^{2\beta_t}q_0^{-2\alpha\beta_t}(1-q_1)^{-2\beta_t +1}\cdot\notag\\
%&&\frac{1}{m^{(\ell)}}\sum_{j=1}^{m^{(\ell)}}\left| \tPsi_s(\zl_j)  \frac{1}{m^{(\ell-1)}}\sum_{i=1}^{m^{(\ell-1)}} w(\zl_j, \zmi_i)\bf^{(\ell-1)}(\zmi_i) -  \gl(\zl_j)     \right|^{2\beta_{t+1}}\notag\\
%&&+  c_0^{2\beta_t}q_1^{-2\beta_t +1}\cdot\notag\\
%&&\frac{1}{m^{(\ell)}}\sum_{j=1}^{m^{(\ell)}}\left| \tPsi_s(\zl_j)  \left[  \frac{1}{m^{(\ell-1)}}\sum_{i=1}^{m^{(\ell-1)}} w(\zl_{j}, \zmi_i)\left(\hf^{(\ell)}(\zmi_i) -  \bf^{(\ell-1)}(\zmi_i)\right) \right]  \right|^{2\beta_t},\notag
%\end{eqnarray}
%where we simply set $q_1 = \frac{1}{4}$ and  $\overset{b}\leq$ uses Jensen Inequality which is
%$$ \left|\frac{1}{m}\sum_{i=1}^m x_i \right|^p \leq  \frac{1}{m}\sum_{i=1}^m \left|x_i\right|^p, ~~ p\geq 1.   $$

%In the following, denote:
%$$
%\Gamma(t, \ell) = \EE \prod_{i=\ell+1}^L\frac{1}{m^{(i)}}\sum_{\ts\in \cA^{\ell+1}}\left|\frac{1}{m^{(\ell)}}\Psi^{(\ell+2)}(\ts)w(z^{\ell+1}_{\ts_{\ell+1}}, \zl_j) \sum^{m^{(\ell)}}_{j=1}\hf^{(\ell)}(\zl_j) - \bf^{(\ell)}(\zl_j)\right|^{2\beta_t},
%$$
%$$
%\Phi(t, \ell) = \EE \prod_{i=\ell+1}^L \frac{1}{m^{(i)}} \sum_{\ts\in \cA^{(\ell)}} \left| 
%\Psi^{(\ell+1)}(\ts)\frac{1}{m^{(\ell-1)}}\sum_{j=1}^{m^{(\ell-1)}}\left[ w(\zl_{\ts_{\ell}},\zmi_{j} )
%\bf^{(\ell-1)}(\zmi_{j}) -  g^{(\ell)}(\zl_{\ts_{\ell}})\right]     \right|^{2\beta_t},
%$$
%and
%$$ d_t = c^{2\beta_t}q_1^{-2\alpha\beta_t-2\beta_t +1}, \quad e_t=  c^{2\beta_t}q_0^{-2\alpha\beta_t}(1-q_1)^{-2\beta_t +1}, \quad  f_t=  c_0^{2\beta_t}q_1^{-2\beta_t +1}.$$

%Note that $\Gamma(0, L-1) =\E |\bf^o-\hf^o |^2$, $\phi(t,l)$ is bounded in \eqref{l use}, $d_t$, $e_t$, and $f_t$ can be treated as constants when $t\leq L$. Then integrating \eqref{ttend} with $s\in \cA^{\ell+1}$, multiplying the both sides by  $\prod_{i=\ell+1}^L\frac{1}{m^{(i)}}$, and taking expectation, for all $\ell\in [2, \dots, L-1]$ and $t\geq 0$, we have
%\begin{eqnarray}
%\Gamma(t, \ell) \leq d_t  \Gamma(t, \ell-1) + e_t  \Phi(t+1, \ell) + f_t \Gamma(t+1, \ell-1).
%\end{eqnarray} 
%For all $t\leq L$, we have
%$$ d_t \leq d_{L}\vee d_{0}, \quad, f_t\leq f_{L}\vee f_{0}.   %  $$
%Let $\gamma = d_{T} \vee f_{T} \vee d_{0} \vee f_{0}$,   for all $t\leq L$, we have
%\begin{eqnarray}
%\Gamma(t, \ell+1) \leq \gamma(\Gamma(t+1, \ell)+ \Gamma(t, \ell)) + \tPhi(t, \ell),
%\end{eqnarray}
%where $ \tPhi(t, \ell) = \Phi(t+1,\ell)e_t$.

%When $\ell=1$, we have  $\Gamma(t, 1)=0$ for all $t\geq 0$. Then we show that 
%\begin{eqnarray}
%\Gamma(t, \ell) \leq \sum_{i=1}^{\ell}\gamma^{\ell-i}\sum_{j=0}^{\ell-i}\left(\begin{matrix}
%\ell-i\\j
%\end{matrix}\right)\tPhi(j+t, i).
%\end{eqnarray}
%We prove it by induction. When $\ell=1$, the above statement is true.  Suppose at $\ell-1$, the statement is true.  We have
%\begin{eqnarray}
%\Gamma(t, \ell+1)&\leq& \sum_{i=1}^{\ell} \gamma^{\ell-i+1} \sum_{j=0}^{\ell-i}\left(\begin{matrix}
%\ell-i\\j
%\end{matrix}\right)\tPhi(j+t+1,i) +\sum_{i=1}^{\ell} \gamma^{\ell-i+1} \sum_{j=0}^{\ell-i}\left(\begin{matrix}
%\ell-i\\j
%\end{matrix}\right)\tPhi(j+t,i)+ \tPhi(t, {\ell+1})\notag\\
%&\overset{a}{=}&\sum_{i=1}^{\ell} \gamma^{\ell-i+1}\left[ \sum_{j=1}^{\ell-i+1}\left(\begin{matrix}
%\ell-i+1\\j
%\end{matrix}\right)\tPhi({j+t}, i)+ \tPhi(t,i)+ \tPhi({\ell-i+1+t},i) \right] +\tPhi(t,{\ell+1})\notag\\
%&=&\sum_{i=1}^{\ell+1}\gamma^{\ell+1-i}\sum_{j=0}^{\ell+1-i}\left(\begin{matrix}
%\ell+1-i\\j
%\end{matrix}\right)\tPhi(j+t, i), \notag
%\end{eqnarray} 
%where in $\overset{a}=$, we use 
%$$ \left(\begin{matrix}
%n\\k
%\end{matrix}\right) +\left(\begin{matrix}
%n\\k+1
%\end{matrix}\right) = \left(\begin{matrix}
%n+1\\k+1
%\end{matrix}\right).$$
%In all, we have
%\begin{eqnarray}
%&&\E| \bf^{o}-\hf^{o}|^2\notag\\
%&=&\Gamma(0, L-1) \notag\\
%& \overset{a}{\leq}&  L\gamma^{L} C^0_{B_T}(c_{M_2} \vee 1)) (e_L\vee e_0) \mathcal{O}\left( \sum_{\ell=1}^{L} \frac{1}{(m^{(j)})^{1+\alpha}} \right)\notag\\
%&\overset{b}{=}&\mathcal{O}\left( \sum_{\ell=1}^{L} \frac{1}{(m^{(j)})^{1+\alpha}} \right)
%\end{eqnarray}
%where in $\overset{a}=$, we use the fact that for all $\Phi(t+1, \ell)$ has the lowest order $\frac{1}{(m^{(j)})^{1+\alpha}}$  only when $t=0$ and $j=0$ and in  $\overset{b}=$, we use both $\gamma$, $C^0_{B_T}$, $e_L$, and $e_0$ only depend on $L, \alpha, c_M,$ and $L$, and can be treated as constants. 


%Furthermore, by setting $\alpha = \mathcal{O}(\frac{1}{L})$, we explictly have
%\begin{eqnarray}
%\E| \bf^{o}-\hf^{o}|^2\leq \mathcal{O}\left(\sum_{\ell=1}^{L} \frac{L(cc_0\vee c^2)^{eL} (c_{M_2} \vee 1)} {(m^{(\ell)})^{1+\mathcal{O}(\frac{1}{L})}} \right).
%\end{eqnarray}

%\end{proof}


%\item  The proof is ended by the fact that
%$$\E| \hf^{o}-  f^{o}|^2\leq 2\E| f^{o}-\bf^{o}|^2 +2\E| \bf^{o}-\hf^{o}|^2. $$


%\end{enumerate}



\subsection{Additional Lemmas}
\begin{lemma}\label{lip}
Suppose $\tilde{h}$ satisfies:
$$| \nabla \tilde{h} (x) -  \nabla \tilde{h} (y) |\leq \tilde{c} | x-y |^{\alpha}$$
with $\alpha> 0$, then we have
\begin{eqnarray}
\left|\tilde{h}(x) - \tilde{h}(y) - \<\nabla \tilde{h}(x), x-y\>   \right| \leq \frac{ \tilde{c}}{1+\alpha}|x-y |^{1+\alpha}\leq \tilde{c}| x - y |^{1+\alpha}.
\end{eqnarray}
\end{lemma}
\begin{proof}
The above argument is right by observing:
\begin{eqnarray}
\left| \tilde{h}(y) - \tilde{h}(x)   - \<\nabla \tilde{h}(x), y-x\>   \right|= \left|\int_{x}^y [\nabla\tilde{h}(t)- \nabla \tilde{h}(x)]dt  \right|\leq \int_{x}^y    \tilde{c} \left|t -x  \right|^{\alpha}dt. \notag
\end{eqnarray}
\end{proof} 

\begin{lemma}\label{jcon}
For all $t\geq1$, for any $t_1\in\RR$, $t_2\in\RR$, $t_3\in \RR$,  $q_1\in (0, 1)$, and $q_2\in (0, 1)$,  we have
\begin{eqnarray}
| t_1 +t_2  |^t \leq \frac{|t_1|^t}{(1-q_1)^{t-1}}+ \frac{|t_2|^t}{(q_1)^{t-1}}.
\end{eqnarray}
and
\begin{eqnarray}\label{jcon1}
| t_1 +t_2 +t_3 |^t \leq \frac{|t_1|^t}{(1-q_2)^{t-1}}+ \frac{|t_2|^t}{(q_2/2)^{t-1}} + \frac{|t_3 |^t}{(q_2/2)^{t-1}}.
\end{eqnarray}
\end{lemma}
\begin{proof}
We prove \eqref{jcon1} only.  Consider function $f(x) = |x|^t$. Because $t\geq1$, $f(x)$ is convex. Thus for any $x_1$, $x_2$, and $x_3$, we have
\begin{eqnarray}
\left|  (1-q_2)x_1 +\frac{q_2}{2}x_2 + \frac{q_2}{2}x_3    \right|^t\leq (1-q_2)|x_1 |^t + \frac{q_2}{2}| x_2|^t + \frac{q_2}{2}|x_3 |^t.
\end{eqnarray} 
Then by setting $x_1 = t_1/(1-q_2)$, $x_2 = 2t_2/q_2$, and $x_3 = 2t_3/q_2$, we can obtain \eqref{jcon1}.



\end{proof}

\begin{lemma}[Rosenthal Inequality]\cite{} \label{rosenthal}
Let $\xi_i$ with $i\in n$ be independent with $\E[\xi_i]=0$ and $\E[|\xi_i |^t]< \infty$ for some $t\geq 2$.  Then we have
$$  \E\left| \sum_{i=1}^n\xi_i \right|^t\leq C^1_t\left(\sum_{i=1}^n \E |\xi_i|^t \right) +C^2_t\left(\sum_{i=1}^n \E [\xi_i^2] \right)^{t/2}, $$
\end{lemma}
where  $C^1_t$ can be take as $(ct)^t$, $C^2_t = (c\sqrt{t})^t$, and $c$ is a constant.

\iffalse
\section{Variance of Discrete Approximation}
\label{apx:discrete-var}

Consider a continuous NN
\[
f(x)=f(\rho,u;x) ,
\]
and let
\[
\hat{f}(x)
\]
be its discrete approximation, where we assume that the approximation is by sampling $m^{(\ell)}$ samples $z^{(\ell)}_j$ from $\rho^{(\ell)}$ for each $\ell$, and set $w^{(\ell)}_{i,j}=w(z^{(\ell)}_i,z^{(\ell-1)}_j)$. 

We have
\[
\hat{g}^{(\ell)}_j(x)=\frac1{m^{(\ell-1)}}\sum_{k=1}^{m^{(\ell-1)}} w^{(\ell)}_{j,k} \hat{f}^{(\ell-1)}_k(x) ,
\]
and
\[
\hat{f}^{(\ell)}_j(x)=h^{(\ell)}(\hat{g}^{(\ell)}_j(x)). 
\]

Similarly, we define
\[
g^{(\ell)}_j(x)=\int w(z^{(\ell)},z^{(\ell-1)}) f^{(\ell-1)}(\z{\ell-1},x)\rho^{(\ell-1)}(\z{\ell-1})\; d \z{\ell-1} , 
\]
and
\[
f^{(\ell)}_j(x)=h^{(\ell)}(g^{(\ell)}_j(x)) .
\]
We also use the convention that
\[
w^{(L+1)}_{i,j}= u_{i,j} ,
\]
and $h^{(L+1)}(g)=g$. 

We also define
\[
\tilde{g}^{(\ell)}_j(x)=\frac1{m^{(\ell-1)}}\sum_{k=1}^{m^{(\ell-1)}} w^{(\ell)}_{j,k} {f}^{(\ell-1)}_k(x) .
\]

\fangcong{
For all $s<\ell\leq L+1$, We can also define for
$$\frac{\partial f^{s}_k (x)}{\partial  \hat{g}_i^{(\ell)}} = \nabla h^{(s)} (g^{(s)}_k (x)) \sum_{j=1}^{m^{(s-1)}} w^{(s)}_{k,j} \frac{\partial f^{s-1}_j (x) }{\partial  \hat{g}_i^{(\ell)}}.$$
Let $\cF^{\ell} = \sigma\{z^{(\ell)}, \dots, z^{(L)}  \}$ be the filtration involving the full random information on the top $L-\ell+1$ layers, where $\sigma$  denotes the sigma field. We can find  that $\frac{\partial f^{s}_k (x)}{\partial  \hat{g}_i^{(\ell)}}$ is measurable on $\sigma\{z^{(\ell)}, \dots, z^{(L)} \}$. 
}
We have the following result.
\begin{lemma}
If $h^{(\ell)}(\cdot)$ are smooth functions with bounded second order derivatives. Then
we have the following expression
\begin{align}
\hat{f}^{(s)}_k(x)
=& f^{(s)}_k(x) 
+ \sum_{\ell=1}^{s-1} \frac{1}{m^{(\ell)}}\sum_{i=1}^{m^{(\ell)}} \frac{\partial \fangcong{f}^{(s)}_k(x)}{\partial \hat{g}^{(\ell)}_i(x)}  (\tilde{g}^{(\ell)}_i(x)-g^{(\ell)}_i(x)) \label{eq:discretize-f}\\
& \; + \nabla h^{(s)}(\fangcong{g}^{(s)}_k(x)) (\tilde{g}^{(s)}_k(x)-{g}^{(s)}_k(x))
+ O\left(\sum_{\ell} \frac{1}{m^{(\ell)}} \sum_{i=1}^{m^{(\ell)}} |\tilde{g}^{(\ell)}_i(x)-g^{(\ell)}_i(x)|^2\right) ,\nonumber
\end{align}
where $\nabla h(\cdot)$ denotes the derivative of $h(\cdot)$.
\end{lemma}
\begin{proof}
We prove by induction. The statement is true when $\ell=1$.  Assume at $\ell-1$, the statement is true.  Now consider layer $\ell$.

Note that by Taylor-expansion, we have
\begin{align*}
\hat{f}^{(\ell)}_k(x)
=& f^{(\ell)}_k(x) 
+ \nabla h^{(\ell)}(g^{(\ell)}_k(x)) (\hat{g}^{(\ell)}_k(x)-\tilde{g}^{(\ell)}_k(x))\\
&+ \nabla h^{(\ell)}(g^{(\ell)}_k(x)) (\tilde{g}^{(\ell)}_j(x)-{g}^{(\ell)}_k(x))+ 
O\left(\sum_{\ell} \frac{1}{m^{(\ell)}} \sum_{i=1}^{m^{(\ell)}} |\tilde{g}^{(\ell)}_i(x)-g^{(\ell)}_i(x)|^2\right)\\
=& f^{(\ell)}_k(x) 
+ \nabla h^{(\ell)}(g^{(\ell)}_k(x))
\frac1{m^{(\ell-1)}}\sum_{j=1}^{m^{(\ell-1)}} w^{(\ell)}_{k,j} (\hat{f}^{(\ell-1)}_j(x)-f^{(\ell-1)}_j(x))
\\
&+ \nabla h^{(\ell)}(g^{(\ell)}_k(x)) (\tilde{g}^{(\ell)}_k(x)-{g}^{(\ell)}_k(x))+ 
O\left(\sum_{\ell} \frac{1}{m^{(\ell)}} \sum_{i=1}^{m^{(\ell)}} |\tilde{g}^{(\ell)}_i(x)-g^{(\ell)}_i(x)|^2\right)
  .
\end{align*}
We can apply \eqref{eq:discretize-f} to $\hat{f}^{(\ell-1)}_j(x)-f^{(\ell-1)}_j(x)$, and obtain
\begin{align*}
\hat{f}^{(\ell)}_k(x)
=& f^{(\ell)}_k(x) 
+ \nabla h^{(\ell)}(g^{(\ell)}_k(x))
\frac1{m^{(\ell-1)}}\sum_{j=1}^{m^{(\ell-1)}} w^{(\ell)}_{k,j}\nabla h^{(\ell-1)}(g^{(\ell-1)}_j) (\tilde{g}^{(\ell-1)}_j(x)-g^{(\ell-1)}_j(x))\\
&+ \nabla h^{(\ell)}(g^{(\ell)}_k(x))
\frac1{m^{(\ell-1)}}\sum_{j=1}^{m^{(\ell-1)}} w^{(\ell)}_{k,j}
\sum_{q=1}^{\fangcong{\ell-2}} 
\frac{1}{m^{(q)}} \sum_{i=1}^{m^{(q)}}
\frac{\partial \fangcong{f}^{(\ell-1)}_j(x)}{\partial \hat{g}^{(q)}_i(x)}  (\tilde{g}^{(q)}_i(x)-g^{(q)}_i(x))
\\
&+ \nabla h^{(\ell)}(g^{(\ell)}_k(x)) (\tilde{g}^{(\ell)}_k(x)-{g}^{(\ell)}_k(x))+ 
O\left(\sum_{\ell} \frac{1}{m^{(\ell)}} \sum_{i=1}^{m^{(\ell)}} |\tilde{g}^{(\ell)}_i(x)-g^{(\ell)}_i(x)|^2\right)
 \\
=& f^{(\ell)}_k(x) 
+ 
\frac1{m^{(\ell-1)}}\sum_{j=1}^{m^{(\ell-1)}} \nabla h^{(\ell)}(\hat{g}^{(\ell)}_k(x)) w^{(\ell)}_{k,j}\nabla h^{(\ell-1)}(\hat{g}^{(\ell-1)}_j) (\tilde{g}^{(\ell-1)}_j(x)-g^{(\ell-1)}_j(x))\\
&+ 
\sum_{q=1}^{\fangcong{\ell-2}} 
\frac{1}{m^{(q)}}
\sum_{i=1}^{m^{(q)}}
\nabla h^{(\ell)}(\fangcong{g}^{(\ell)}_k(x))
\frac1{m^{(\ell-1)}}\sum_{j=1}^{m^{(\ell-1)}} w^{(\ell)}_{k,j}
\frac{\partial \hat{f}^{(\ell-1)}_j(x)}{\partial \hat{g}^{(q)}_i(x)}  (\tilde{g}^{(q)}_i(x)-g^{(q)}_i(x))
\\
&+ \nabla h^{(\ell)}(\fangcong{g}^{(\ell)}_k(x)) (\tilde{g}^{(\ell)}_k(x)-{g}^{(\ell)}_k(x))+ 
O\left(\sum_{\ell} \frac{1}{m^{(\ell)}} \sum_{i=1}^{m^{(\ell)}} |\tilde{g}^{(\ell)}_i(x)-g^{(\ell)}_i(x)|^2\right)
\\
=& f^{(\ell)}_k(x) + 
\sum_{q=1}^{\ell-1} 
\frac{1}{m^{(q)}}
 \sum_{i=1}^{m^{(q)}}
\frac{\partial \fangcong{f}^{(\ell)}_k(x)}{\partial \hat{g}^{(q)}_i(x)}  (\tilde{g}^{(q)}_i(x)-g^{(q)}_i(x))
\\
&+ \nabla h^{(\ell)}(\fangcong{g}^{(\ell)}_k(x)) (\tilde{g}^{(\ell)}_k(x)-{g}^{(\ell)}_k(x))+ 
O\left(\sum_{\ell} \frac{1}{m^{(\ell)}} \sum_{i=1}^{m^{(\ell)}} |\tilde{g}^{(\ell)}_i(x)-g^{(\ell)}_i(x)|^2\right)
 .
\end{align*}
This finishes the proof.
\end{proof}

We are now ready to prove the desired result. From \eqref{eq:discretize-f}, we have
$$ \E\left[  \frac{\partial f^{(s)}_k(x)}{\partial \hat{g}^{(\ell)}_i(x)}  (\tilde{g}^{(\ell)}_i(x)-g^{(\ell)}_i(x))  \right] =\E\left[ \frac{\partial f^{(s)}_k(x)}{\partial \hat{g}^{(\ell)}_i(x)}  \E(\tilde{g}^{(\ell)}_i(x)-g^{(\ell)}_i(x) | \cF^{\ell}) \right]=0. $$
So $\hat{f}(x)$ is an approximately an unbiased estimator of $f(x)$ up to the leading order.  We have the Lemma below to bound the variance of $\hat{f}(x)$:
\begin{lemma}
 If $h^{(\ell)}(\cdot)$ are smooth functions with bounded second order derivatives. We have
 \begin{eqnarray}
 &&\E_{z}\E_x\| \hat{f}(x) - f(\x)\|^2\\
 &\leq& 2(L+1) \sum_{\ell=1}^{L+1}\frac{1}{(m^{(\ell-1)})^2} \sum_{j=1}^{m^{(\ell-1)}} \E_{z}\E_x \left( \frac{1}{m^{(\ell)}}\sum_{i=1}^{m^{(\ell)}} c_{ij}^{(\ell)} w_{i,j}^{(\ell)}  \right)^2 +  O\left(\sum_{\ell} \frac{1}{m^{(\ell)^2}}...\right).\notag
 \end{eqnarray}
\end{lemma}



\fangcong{Left it to me. I will finish it tomorrow.}
\begin{eqnarray}
123
\end{eqnarray}
\fi


\section{Appendix}
\begin{lemma}\label{property of convex}
 $\frac{x^{a}}{y^b}$ is convex on $(x,y)\in [0, +\infty)\times (0, +\infty)  $ when $a-1\geq b  \geq 0$ and is strictly convex on $(x,y)\in (0, +\infty)\times (0, +\infty)$ when $a-1> b \geq 0$.
\end{lemma}
\begin{proof}
When $b=0$, Lemma \ref{property of convex} is right. When $b>0$, let $f(x, y) = \frac{x^a}{y^b},$ we have $  \nabla_x^2 f= \frac{a(a-1)x^{(a-2)}}{y^b}$, $ \nabla_y^2 f= \frac{b(b+1)x^a}{y^{b+2}} $, and $\nabla^2_{xy} f =\frac{ab x^{a-1}}{y^{b+1}}$.  We prove Lemma \ref{property of convex} by showing that for all $x_1 \in \RR$ and $y_1\in \RR$,  
\begin{eqnarray}
\frac{a(a-1)x^{(a-2)}}{y^b}x_1^2  -  2\frac{ab x^{a-1}}{y^{b+1}} x_1y_1 +  \frac{b(b+1)x^a}{y^{b+2}} y_1^2\geq  \ep  \frac{a(a-1)x^{(a-2)}}{y^b}x_1^2 + \ep  \frac{b(b+1)x^a}{y^{b+2}} y_1^2.
\end{eqnarray}
 When $\ep=0$, it is the not-strictly convex case.  The above argument is equivalent to prove that 
\begin{eqnarray}
[a(a-1)-\ep]x_1^2 - 2ab\frac{x}{y}x_1y_1+(b(b+1)-\ep)\frac{x^2}{y^2}y_1^2\geq 0.
\end{eqnarray}
Furthermore, it is sufficient to obtain that 
\begin{eqnarray}\label{con tte}
[a(a-1)-\ep][ b(b+1)-\ep ]\geq a^2b^2.
\end{eqnarray}
Set  $\ep_1=a-b-1\geq0$, $\ep = \frac{ab\ep_1}{b^2+b+a^2 -a}$, $\ep_a = \ep/a$, and $\ep_b = \ep/b$. We have
$$  \ep_1\geq  \ep_a(b+1) +(a-1)\ep_b -\ep_a \ep_b, $$ 
which leads to \eqref{con tte}.
\end{proof}

\section{Proof of Theorem \ref{thm:nfr}}
\begin{proof} The statement is true when $\ell=0$ if we  let $\Q{0}$ be the identity mapping.
  Assume the statement is true for $\ell-1$. We have
\[
\ff^{(\ell-1)}(\rho,\z{\ell-1},x)  
=\ff^{(\ell-1)}(\rhoo,\tilde{z}^{(\ell-1)},x) .
\]
Recall that the map
$\Q{\ell}(\tilde{\rho},\rho_0;\cdot): \cZ{\ell} \to \cZ{\ell}$ takes the form of:
\begin{equation}
\Q{\ell}(\tilde{\rho},\rho_0;z)(\Q{\ell}(\tilde{\rho},\rho_0;\zeta)) = \z{\ell}(\zeta)
\frac{d\tilde{\rho}^{(\ell-1)}(\Q{\ell}(\tilde{\rho},\rho_0;\zeta))}{d\rhoo^{(\ell-1)}(\Q{\ell}(\tilde{\rho},\rho_0;\zeta))} .
\label{eq:nfr-Q}
\end{equation}
Now, the distribution $\rho^{(\ell)}(\cdot)$ on $\z{\ell}$ induces a
distribution $\tilde{\rho}^{(\ell)}(\cdot)$ on $\tz{\ell}=\Q{\ell}(\z{\ell})$.


In the following derivation, we let $\tz{\ell}=\Q{\ell}(\z{\ell})$ and $\tz{\ell-1}=\Q{\ell-1}(\z{\ell-1})$.
Then for the case of $\ell$, it follows that
\begin{align*}
\ff^{(\ell)}(\rho,\z{\ell},x) =&
h^{(\ell)}\left( \int
  w(\z{\ell}, \z{\ell-1}) \ff^{(\ell-1)}(\rho,\z{\ell-1},x)
  d{\rho}^{(\ell-1)}(\z{\ell-1})\right)\\
=&
h^{(\ell)}\left( \int
  w(\z{\ell}, \z{\ell-1}) \ff^{(\ell-1)}(\rhoo,\tz{\ell-1},x)
  d{\rho}^{(\ell-1)}(\z{\ell-1})\right)\\
 =&
h^{(\ell)}\left( \int
  w(\z{\ell}, \z{\ell-1}) \ff^{(\ell-1)}(\rhoo,\tz{\ell-1},x)
  d\tilde{\rho}^{(\ell-1)}(\tz{\ell-1})\right)\\ 
  =&
h^{(\ell)}\left( \int
  w(\z{\ell}, \z{\ell-1}) \ff^{(\ell-1)}(\rhoo,\tz{\ell-1},x)
  \frac{d\tilde{\rho}^{(\ell-1)}(\tz{\ell-1})}{d\rhoo(\tilde{z}^{(\ell-1)})}d\rhoo^{(\ell-1)}(\tilde{z}^{(\ell-1)})\right)\\ 
  =&
h^{(\ell)}\left( \int
  w(\tz{\ell}, \tz{\ell-1}) \ff^{(\ell-1)}(\rhoo,\tz{\ell-1},x)
  d\rhoo^{(\ell-1)}(\tilde{z}^{(\ell-1)})\right)\\
  =& \ff^{(\ell)}(\rhoo,\tz{\ell},x) .
\end{align*}
Therefore, the statement holds for all $\ell \in \{1,...,L\}$.

We let $\tu = \tau^{u}(\tilde{\rho},\rho_0;u)$. Then from the definition of $\tau^{u}(\tilde{\rho},\rho_0;\cdot)$, we have,
\begin{align}
\tu(\Q{L}(\tilde{\rho},\rho_0;\zeta))=
u(\zeta) \frac{d\tilde{\rho}^{(L)}}{d\rhoo^{(L)}}(\Q{L}(\tilde{\rho},\rho_0;\zeta)),\nonumber
\end{align}
for $\zeta \in \cZ{L}$.

Therefore, for the top layer, 
let $\tz{L}=\Q{L}(\z{L})$,
we have
\begin{align*}
\ff(\rho,\u,x) =&  \int
  \u(\z{L}) \ff^{(L)}(\rho,\z{L},x)
  d\rho^{(L)}(\z{L}) \\
  =&\int
  \u(\z{L}) \ff^{(L)}(\rhoo,\tz{L},x)
  d\tilde{\rho}^{(L)}(\tz{L})\\
  =&\int
  \u(\z{L}) \ff^{(L)}(\rhoo,\tz{L},x)
  \frac{d\tilde{\rho}^{(L)}(\tz{L})}{d\rhoo^{(L)}(\tz{L})}d\rhoo^{(L)}(\tz{L})\\
  =&\int
  \tu(\tz{L}) \ff^{(L)}(\rhoo,\tz{L},x)
  d \rhoo^{(L)}(\tz{L})\\
    =& \ff(\rhoo,\tu,x).
\end{align*}


For the regularizer, we have
\begin{align}
R^{(\ell)}(\rho)&=\int r_2\left (\int r_1\Big(w (z^{(\ell)}, z^{(\ell-1)})\Big)d\rho^{(\ell)}(z^{(\ell)})\right ) d\rho^{(\ell-1)}(z^{(\ell-1)})\nonumber\\
&=\int r_2\left (\int r_1\Big(w (z^{(\ell)}, z^{(\ell-1)})\Big)d\tilde{\rho}^{(\ell)}(\tilde{z}^{(\ell)})\right ) d\tilde{\rho}^{(\ell-1)}(\tilde{z}^{(\ell-1)})\nonumber\\
&=\int r_2\left (\int r_1\Big(w (\tilde{z}^{(\ell)}, \tilde{z}^{(\ell-1)})\frac{d\rhoo^{(\ell-1)}}
{d\tilde{\rho}^{(\ell-1)}}(\tz{\ell-1})\Big)d\tilde{\rho}^{(\ell)}(\tilde{z}^{(\ell)})\right ) d\tilde{\rho}^{(\ell-1)}(\tilde{z}^{(\ell-1)})\nonumber
\end{align}

%\begin{align*}
%R^{(\ell)}(\rho,u)=& \int \int [w(\z{\ell},\z{\ell-1})]^{q_\ell} d\rho^{(\ell)}(\z{\ell})d\rho^{(\ell-1)}(\z{\ell-1})\\
%=& \int \int [w(\z{\ell},\z{\ell-1})]^{q_\ell} d\tilde{\rho}^{(\ell)}(\tz{\ell})d\tilde{\rho}^{(\ell-1)}(\tz{\ell-1})\\
%=& \int \int \left[
%w(\tz{\ell},\tz{\ell-1})
%\frac{d\rhoo^{(\ell-1)}}
%{d\tilde{\rho}^{(\ell-1)}}(\tz{\ell-1})
%\right]^{q_\ell} d\tilde{\rho}^{(\ell)}(\tz{\ell})d\tilde{\rho}^{(\ell-1)}(\tz{\ell-1})\\
%=&\int \int \left[
%w(\tz{\ell},\tz{\ell-1})
%\right]^{q_\ell} \frac{d\tilde{\rho}^{(\ell)}(\tz{\ell})/d\rhoo^{\ell}(\tz{\ell})}{\big(d\tilde{\rho}^{(\ell-1)}(\tz{\ell-1})/d\rhoo^{(\ell-1)}(\tz{\ell-1})\big)^{q_\ell-1}}d\rhoo^{(\ell-1)}(\tz{\ell-1})d\rhoo^{(\ell)}(\tz{\ell})
%\end{align*}
Moreover,
\begin{align}
R^{(\u)}(\rho,\u) &=  \int r^{(u)}(\u(z^{(L)}))
                 d\rho^{(L)}(z^{(L)})\nonumber\\
                 &=\int r^{(u)}(\u(z^{(L)}))
                 d\tilde{\rho}^{(L)}(\tilde{z}^{(L)})\nonumber\\
                 &=\int r^{(u)}\Big(\tu(\tz{L})\frac{d\rhoo^{(L)}}{d\tilde{\rho}^{(L)}}(\tz{L})\Big)
                 d\tilde{\rho}^{(L)}(\tilde{z}^{(L)}).\nonumber
\end{align}
%\begin{align*}
%R^{(\u)}(\rho,\u) =&  \int \|\u(\z{L})\|^{q_u}
%       d\rho^{(L)}(\z{L})\\
%       =&\int \|\u(\z{L})\|^{q_u}
%       d\tilde{\rho}^{(L)}(\tz{L})\\
%       =&\int \left\|\tu(\tz{L})\frac{d\rhoo^{(L)}}{d\tilde{\rho}^{(L)}}(\tz{L})\right\|^{q_u}
%       d\tilde{\rho}^{(L)}(\tz{L})\\
%       =&\int \frac{\|\tu(\tz{L})\|^{q_u}}{\big(d\tilde{\rho}^{(L)}(\tz{L})/d\rhoo^{(L)}(\tz{L})\big)^{q_u-1}}
%       d\rhoo^{(L)}(\tz{L}).
%\end{align*}
This proves the desired result.
\end{proof}

\section{Proof of Theorem \ref{thm:nfr-inv}}
\begin{proof} of Theorem \ref{thm:nfr-inv}:

 $\rho^{(\ell)}$ can be recovered by the inverse of the mapping $\Q{\ell}(\tilde{\rho},\rho_0;\cdot)$, i.e., $\tilde{\tau}^{(\ell)}(\tilde{\rho},\rho_0;\cdot)$,  recursively. That is  we can define $\rho^{(\ell)}$ recursively such that the probability distribution $\tilde{\rho}^{(\ell)}$ on $\tz{\ell}$ induces a probability distribution $\rho^{(\ell)}$ on $\z{\ell}=\tQ{\ell}(\tilde{\rho},\rho_0; \tz{\ell})$. $u$ can be be recovered by 
  \[
  u = \tilde{\tau}^{u}(\tilde{\rho}, \rho_0;\tilde{u}).\nonumber
  \]
  The remaining of the proof is identical to that of Theorem~\ref{thm:nfr}.
\end{proof}

%\section{Proof of Theorem \ref{thm:nfr}}
%\begin{proof} The statement is true when $\ell=0$ if we  let $\Q{0}$ be the identity mapping.
%  Assume the statement is true for $\ell-1$. We have
%\[
%\ff^{(\ell-1)}(\rho,\z{\ell-1},x)  
%=\ff^{(\ell-1)}(\rho_0,\tilde{z}^{(\ell-1)},x) .
%\]
%We can now define the mapping
%$\Q{\ell}: \cZ{\ell} \to \cZ{\ell}$ as follows:
%\begin{equation}
%\Q{\ell}(z)(\Q{\ell-1}(\zeta)) = \z{\ell}(\zeta)
%\frac{\tilde{\rho}^{(\ell-1)}(\Q{\ell-1}(\zeta))}{\rho_0^{(\ell-1)}(\Q{\ell-1}(\zeta))} .
%\label{eq:nfr-Q}
%\end{equation}
%Now, the distribution $\rho^{(\ell)}(\cdot)$ on $\z{\ell}$ induces a
%distribution $\tilde{\rho}^{(\ell)}(\cdot)$ on $\tz{\ell}=\Q{\ell}(\z{\ell})$.


%In the following derivation, we let $\tz{\ell}=\Q{\ell}(\z{\ell})$ and $\tz{\ell-1}=\Q{\ell-1}(\z{\ell-1})$.
%Then for the case of $\ell$, it follows that
%\begin{align*}
%\ff^{(\ell)}(\rho,\z{\ell},x) =&
%h^{(\ell)}\left( \int
%  w(\z{\ell}, \z{\ell-1}) \ff^{(\ell-1)}(\rho,\z{\ell-1},x)
%  {\rho}^{(\ell-1)}(\z{\ell-1}) d \z{\ell-1}\right)\\
%=&
%h^{(\ell)}\left( \int
%  w(\z{\ell}, \z{\ell-1}) \ff^{(\ell-1)}(\rho_0,\tz{\ell-1},x)
%  {\rho}^{(\ell-1)}(\z{\ell-1}) d \z{\ell-1}\right)\\
% =&
%h^{(\ell)}\left( \int
%  w(\z{\ell}, \z{\ell-1}) \ff^{(\ell-1)}(\rho_0,\tz{\ell-1},x)
%  \tilde{\rho}^{(\ell-1)}(\tz{\ell-1}) d \tz{\ell-1}\right)\\ 
%  =&
%h^{(\ell)}\left( \int
%  w(\tz{\ell}, \tz{\ell-1}) \ff^{(\ell-1)}(\rho_0,\tz{\ell-1},x)
%  {\rho}_0^{(\ell-1)}(\tz{\ell-1}) d \tz{\ell-1}\right)\\
%  =& \ff^{(\ell)}(\rho_0,\tz{\ell},x) .
%\end{align*}
%Therefore, the statement holds for all $\ell \in \{1,...,L\}$.

%For the top layer, 
%let $\tz{L}=\Q{L}(\z{L})$,
%we have
%\begin{align*}
%\ff(\rho,\u,x) =&  \int
%  \u(\z{L}) \ff^{(L)}(\rho,\z{L},x)
%  \rho^{(L)}(\z{L}) d \z{L} \\
%  =&\int
%  \u(\z{L}) \ff^{(L)}(\rho_0,\tz{L},x)
%  \tilde{\rho}^{(L)}(\tz{L}) d \tz{L}\\
%  =&\int
%  \tu(\tz{L}) \ff^{(L)}(\rho_0,\tz{L},x)
%  \rho_0^{(L)}(\tz{L}) d \tz{L}\\
%    =& \ff(\rho_0,\tu,x) ,
%\end{align*}
%where we define
%\[
%\tu(\Q{L}(\zeta))=
%u(\zeta) \frac{\tilde{\rho}^{(L)}(\Q{L}(\zeta))}{\rho_0^{(L)}(\Q{L}(\zeta))}
%\]
%for $\zeta \in \cZ{L}$.

%For the regularizer, we have
%\begin{align*}
%R^{(\ell)}(\rho,u)=& \int \int [w(\z{\ell},\z{\ell-1})]^{q_\ell} {\rho}^{(\ell)}(\z{\ell})\rho^{(\ell-1)}(\z{\ell-1})d \z{\ell} d \z{\ell-1}\\
%=& \int \int [w(\z{\ell},\z{\ell-1})]^{q_\ell} \tilde{\rho}^{(\ell)}(\tz{\ell})\tilde{\rho}^{(\ell-1)}(\tz{\ell-1})d \tz{\ell} d \tz{\ell-1}\\
%=& \int \int \left[
%w(\tz{\ell},\tz{\ell-1})
%\frac{\rho_0^{(\ell-1)}(\tz{\ell-1})}
%{\tilde{\rho}^{(\ell-1)}(\tz{\ell-1})}
%\right]^{q_\ell} \tilde{\rho}^{(\ell)}(\tz{\ell})\tilde{\rho}^{(\ell-1)}(\tz{\ell-1})d \tz{\ell} d \tz{\ell-1} \\
%=& \int \int 
%w(\tz{\ell},\tz{\ell-1})^{q_\ell}
%\frac{\rho_0^{(\ell-1)}(\tz{\ell-1})^{q_\ell}}
%{\tilde{\rho}^{(\ell-1)}(\tz{\ell-1})^{q_\ell-1}}
% \tilde{\rho}^{(\ell)}(\tz{\ell}) d \tz{\ell} d \tz{\ell-1} .
%\end{align*}
%Moreover,
%\begin{align*}
%R^{(\u)}(\rho,\u) =&  \int \|\u(\z{L})\|^{q_u}
%       \rho^{(L)}(\z{L}) d \z{L} \\
%       =&\int \|\u(\z{L})\|^{q_u}
%       \tilde{\rho}^{(L)}(\tz{L}) d \tz{L} \\
%       =&\int \left\|\tu(\tz{L})\frac{\rho_0^{(L)}(\tz{L})}{\tilde{\rho}^{(L)}(\tz{L})}\right\|^{q_u}
%       \tilde{\rho}^{(L)}(\tz{L}) d \tz{L}\\
%       =&\int \frac{\|\tu(\tz{L})\|^{q_u}}{\tilde{\rho}^{(L)}(\tz{L})^{q_u-1}}
%       {\rho}_0^{(L)}(\tz{L})^{q_u} d \tz{L} .
%\end{align*}
%This proves the desired result.
%\end{proof}

\section{Proof og Theorem \ref{thm:convexity}}
\begin{proof}
Let $$t_1^{(\ell)}(z^{(\ell)}) = \frac{d\tilde{\rho}(z^{(\ell)})}{d \rho_0(z^{(\ell)})}, \quad \ell \in [L].$$
It is equivalent to prove that $\tilde{Q}(\tilde{\rho}, \tilde{u})$ is convex on $(t_1, \tilde{u})$.  From \eqref{eq:nfr-j}, \eqref{eq:nfr-r-layer}, and \eqref{eq:nfr-r-top}, we have 
\begin{align}
    &\tilde{Q}(\tilde{\rho},\tu)\notag\\
    =&  J(\ff(\rho_0,\tu,\cdot)) + \lambda^{(u)} \int \Big\| \frac{\tu (\tilde{z}^{(L)})}{t_1^{(L)}(\tilde{z}^{(L)})} \Big\|^2t_1^{(L)}(\tilde{z}^{(L)}) d  \rho_0^{(L)}(\tilde{z}^{(L)}) \notag\\
   & +  \sum_{\ell=1}^{L}\lambda^{(\ell)}  \int \left|\int \Big|\frac{w (\tilde{z}^{(\ell)}, \tilde{z}^{(\ell-1)})}
{t_1^{(\ell-1)}(\tilde{z}^{(\ell-1)})}\Big| t_1^{(\ell)}(\tilde{z}^{(\ell)}) d\rho_0^{(\ell)}(\tilde{z}^{(\ell)})\right|^2 t_1^{(\ell-1)}(\tilde{z}^{(\ell-1)}) d\rho_0^{(\ell-1)}(\tilde{z}^{(\ell-1)})\notag\\
=& \underbrace{J(\ff(\rho_0,\tu,\cdot))}_{I_1} + \lambda^{(u)}\underbrace{ \int \frac{\|\tu (\tilde{z}^{(L)})\|^2}{t_1^{(L)}(\tilde{z}^{(L)})}  d  \rho_0^{(L)}(\tilde{z}^{(L)})}_{I_2} \notag\\
   & +  \sum_{\ell=1}^{L}\lambda^{(\ell)}   \int\underbrace{ \frac{\left|\int\Big|w (\tilde{z}^{(\ell)}, \tilde{z}^{(\ell-1)}) \Big| t_1^{(\ell)}(\tilde{z}^{(\ell)}) d\rho_0^{(\ell)}(\tilde{z}^{(\ell)})\right|^2}{t_1^{\ell-1}(\tilde{z}^{(\ell-1)})}}_{I_3^{(\ell)}}  d\rho_0^{(\ell-1)}(\tilde{z}^{(\ell-1)}).\notag\\
\end{align}
$I_1(\tu)$ is convex  on $\tu$ under our assumption that $\phi$ is convex.  $I_2(\tu, t_1^{(L)})$ is convex on $(\tu, t_1^{(L)})$ from Lemma \ref{property of convex}.  Besides, $I_3^{(\ell)}(t_1^{\ell})$  with $\ell \in [L]$ are  in the form of the square of sums and thus are  also convex on $t_1^{\ell}$.  So $\tilde{Q}$ is convex on $(t_1,\tu)$, which finishes the proof.

We can introduce $t_2^{\ell-1}(\tilde{z}^{\ell-1})= \int\Big|w (\tilde{z}^{(\ell)}, \tilde{z}^{(\ell-1)}) \Big| t_1^{(\ell)}(\tilde{z}^{(\ell)}) d\rho_0^{(\ell)}(\tilde{z}^{(\ell)})$.

$$I_3^{\ell}  =  \frac{\left|t_2^{\ell-1}(\tilde{z}^{\ell-1})\right|^2}{t_1^{\ell-1}(\tilde{z}^{(\ell-1)})}  $$




\end{proof}


\section{Proof of Theorem \ref{theorem:global-optimum}}
\begin{proof} of Theorem \ref{theorem:global-optimum}:\\
Consider the problem:
\begin{eqnarray}
&&\min_{\tilde{\rho}} ~~ \tilde{Q}(\tilde{\rho}, \tilde{u})\notag\\
&&s.t.~~\trho^{(\ell)}\geq 0  ~\text{and}~ \int \trho^{(\ell)}(z^{(\ell)})d z^{(\ell)} = 1, ~\ell \in \{1, \dots, L \}. \notag
\end{eqnarray}
Let $a_0 = 1$, $b_1 = a_0\geq1$, and $b_{\ell+1} = b_{\ell}(q_{\ell}-1)+a_0\geq1$ for all $\ell \in\{2, \dots, L-1\}$.
We can change  variable $t$  as $\trho^{(\ell)} = (t^{(\ell)})^{b_{\ell}}\rho_0^{(\ell)}$ for all $\ell \in \{1, \dots,  L\}$. Then it is equivalent to solve the problem:
\begin{eqnarray}\label{t problem}
&&\min_{t}~~\sum_{\ell=1}^L \lambda^{(\ell)} \bar{R}^{(\ell)}(t, \tu) +\lambda^{(u)}\bar{R}^{(u)}(t, \tu) \\
&&s.t.~~t^{(\ell)}\geq 0  ~\text{and}~ \int  t^{(\ell)}(z^{(\ell)})^{b_{\ell}} \rho_0^{(\ell)}(z^{(\ell)})d z^{(\ell)} = 1, ~\ell \in \{1, \dots, L\}, \notag
\end{eqnarray}
where 
$$  
\bar{R}^{(\ell)}(t,\tu)=\int \int 
w(\tz{\ell},\tz{\ell-1})^{q_\ell}
\frac{\rho_0^{(\ell-1)}(\tz{\ell-1})\rho_0^{(\ell)}(\tz{\ell})}
{t^{(\ell-1)}(\tz{\ell-1})^{b_{\ell-1}(q_\ell-1)}}
 t^{(\ell)}(\tz{\ell})^{b_{\ell-1}(q_\ell-1)+a_0} d \tz{\ell} d \tz{\ell-1}
$$
and 
$$
 R^{(u)}(t,\tu)= \int \frac{\|\tu(\tz{L})\|^{q_u}}{t^{(L)}(\tz{L})^{b_L (q_u-1)}}
       {\rho}_0^{(L)}(\tz{L}) d \tz{L} .
$$
Because $f(x, y) = \frac{x^{a}}{y^{b}}$ with $b\geq a-1\geq1$ is joint convex on $x,y$ (Refer the proof in Lemma \ref{property of convex}), the objective  of \eqref{t problem} is a convex function.  Since  $b_\ell\geq1$,   the weighted $\ell$-$b_\ell$ norm is also convex.  We can relax  problem \eqref{t problem}  to following convex optimization problem:
\begin{eqnarray}\label{problemt}
&&\min_{t}~~\sum_{\ell=1}^L \lambda^{(\ell)} \bar{R}^{\ell}(t, \tu) +\lambda^{(u)}\bar{R}^{(u)}(t, \tu) \\
&&s.t.~~t^{(\ell)}\geq 0  ~\text{and}~ \int  t^{(\ell)}(\tilde{z}^{(\ell)})^{b_{\ell}} \rho_0^{(\ell)}(\tilde{z}^{(\ell)})d \tilde{z}^{(\ell)} \leq 1, ~~\ell \in \{1, \dots, L\}, \notag
\end{eqnarray}
  Let $t_*$ satisfies  $t_*^{\ell} = (\trho^{(\ell)}_* /\rho_0^{(\ell)})^{\frac{1}{b_\ell}} $ for all $\ell \in \{1, \dots, L\}$.  We show $t_*$ is  the minimum solution of  \eqref{problemt}. To achieve it, using that  $\trho_*$ satisfies the KKT conditon for \eqref{tilderho}, there exist  real number sequences of $\{\Lambda_1^{(\ell)}\}_{\ell = 1, \dots, L}$ and $\{\Lambda_2^{(\ell)}\}_{\ell = 1, \dots, L}$  such that 
\begin{eqnarray}
&&\lambda^{(1)}\nabla_{\trho^{(1)}}\tilde{R}^{(1)}(\trho_*, \tu) +\Lambda_1^{(1)}+\Lambda_2^{(1)} = 0, \label{KKT 1} \notag\\
&&\lambda^{(\ell+1)}\nabla_{\trho^{(\ell)}}\tilde{R}^{(\ell+1)}(\trho_*, \tu)+ \lambda^{(\ell)}\nabla_{\trho^{(\ell)}}\tilde{R}^{(\ell)}(\trho_*, \tu)+\Lambda^{(\ell)}_1+\Lambda^{(\ell)}_2 = 0,~~ \ell \in  \{2, \dots, L-1\},\notag \label{KKT 2}\\
&&\lambda^{(L)}\nabla_{\trho^{(L)}}\tilde{R}^{(L)}(\trho_*, \tu)+ \lambda^{(u)}\nabla_{\trho^{(L)}}\tilde{R}^{(u)}(\trho_*, \tu)+\Lambda^{(L)}_1+\Lambda^{(L)}_2= 0,  \label{KKT 3}\\
&&\Lambda^{(\ell)}_1\trho_*^{(\ell)} = 0, ~ \Lambda^{(\ell)}_1\leq 0, ~ \trho_*^{(\ell)}\geq 0,~~  \ell \in  \{1, \dots, L\},\notag\\
&& \int \trho_*^{(\ell)} d\tilde{z}^{\ell} = 1,~~\ell \in  \{1, \dots, L\}.\notag
\end{eqnarray}
We prove $\Lambda_2^{(\ell)}\geq0$ holds for all $\ell\in \{1, 2, \dots,L\}$.  Let $z^{(\ell)} = 0$ denotes the function which mappings all $z^{(\ell-1)}\in \mathcal{Z}^{(\ell-1)}$ to $0$ with $\ell \in  \{1, \cdots, L\}$. Consider the point $z^{L} = 0$,  from \eqref{KKT 3} we have
$$
- (q_u-1)\lambda^{(u)}\frac{\| \tu(0)\|^{q_u}}{\trho_*^{(L)}(0)^{q_u}} + \Lambda_1^{(L)}+ \Lambda_2^{(L)} =0.
$$
For $\Lambda_1^{(L)}\leq 0$,   we have $\Lambda_2^{(L)}\geq0$.  In a similar way, for all $\ell\in \{1, \dots, L-1\}$, we have
$$
-  q_\ell\lambda^{(\ell+1)} \frac{\int w(\tilde{z}^{(l+1)}, 0)^{q_\ell} \rho_0^{(\ell)}(0)^{(q_\ell)}\trho_*^{(\ell+1)}(\tilde{z}^{\ell+1})d\tilde{z}^{(\ell+1)} }{\trho_*^{\ell}(0)^{q_\ell+1}   } + \Lambda_1^{(\ell)}+ \Lambda_2^{(\ell)} =0,
$$
which indicates that $\Lambda_2^{(\ell)}\geq0$. We denote  
$ \bar{\Lambda}_2^{(\ell)} = \frac{\partial  \trho_*^{(\ell)}}{\partial t_*^{(\ell)}}   {\Lambda}_2^{(\ell)}=   \rho_0^{(\ell)} b_{\ell} (t_*^{(\ell)})^{b_l-1}{\Lambda}_2^{(\ell)}\geq0$ and let $ \bar{\Lambda}_1^{(\ell)} =   \rho_0^{(\ell)} b_{\ell} (t_*^{(\ell)})^{b_l-1}{\Lambda}_1^{(\ell)}\leq 0.$ We have 
\begin{eqnarray}
&&\lambda^{(1)}\nabla_{t^{(1)}}\bar{R}^{(1)}(t_*, \tu) +\bar{\Lambda}_1^{(1)}+\bar{\Lambda}_2^{(1)} = 0, \notag\\
&&\lambda^{(\ell+1)}\nabla_{t^{(\ell)}}\bar{R}^{(\ell+1)}(t_*, \tu)+ \lambda^{(\ell)}\nabla_{t^{(\ell)}}\bar{R}^{(\ell)}(t_*, \tu)+\bar{\Lambda}^{(\ell)}_1+\bar{\Lambda}^{(\ell)}_2 = 0,~~ \ell \in  \{2, \dots, L-1\},\notag \\
&&\lambda^{(L)}\nabla_{t^{(L)}}\bar{R}^{(L)}(t_*, \tu)+ \lambda^{(u)}\nabla_{t^{(L)}}\bar{R}^{(u)}(t_*, \tu)+\bar{\Lambda}^{(L)}_1+\bar{\Lambda}^{(L)}_2= 0, \notag \\
&&\bar{\Lambda}_1^{(\ell)}t_*^{(\ell)} = 0, ~ \bar{\Lambda}_1^{(\ell)}\leq 0, ~ t_*^{(\ell)}\geq 0,~~  \ell \in  \{1, \dots, L\}, \notag\\
&&\int t_*^{(\ell)}(\tilde{z}^{(\ell)})^{b_{\ell}} \rho_0^{(\ell)}(\tilde{z}^{(\ell)})d \tilde{z}^{(\ell)} \leq 1,~~\ell \in  \{1, \dots, L\}, \notag\\
&&\bar{\Lambda}^{(\ell)}_2 \left(\int t_*^{(\ell)}(\tilde{z}^{(\ell)})^{b_{\ell}} \rho_0^{(\ell)}(\tilde{z}^{(\ell)})d \tilde{z}^{(\ell)}- 1\right)=0,~\bar{\Lambda}^{(\ell)}_2\geq0,    ~~\ell \in  \{1, \dots, L\}.\notag
\end{eqnarray}
So  $\left\{ t_*^{(\ell)},\bar{\Lambda}_1^{(\ell)},\bar{\Lambda}_2^{(\ell)}\right\}_{\ell = 1, \dots, L}$ satisfies the KKT condition for the convex optimization problem \eqref{problemt}. Thus it is a global solution for \eqref{problemt}. This implies that it is also  a global solution  for \eqref{t problem}.  We obtain our result.
\end{proof}




\section{Convergence of Neural Feature Repopulation Algorithms}\label{sec:convergence-discussion}
\begin{theorem}
  The feature repopulation process converges to the optimal solution.
\end{theorem}
